# Supplementary material for: How to Probe: Simple Yet Effective Techniques for Improving Post-hoc Explanations
Source: arXiv:2503.00641 source file (2025-03-01)
Supplement: Supplementary file 1 [file bce_vs_ce_in1k_quanti.tex]

\begin{figure*}
\begin{center}
    \centering
    \includegraphics[width=.90\linewidth]{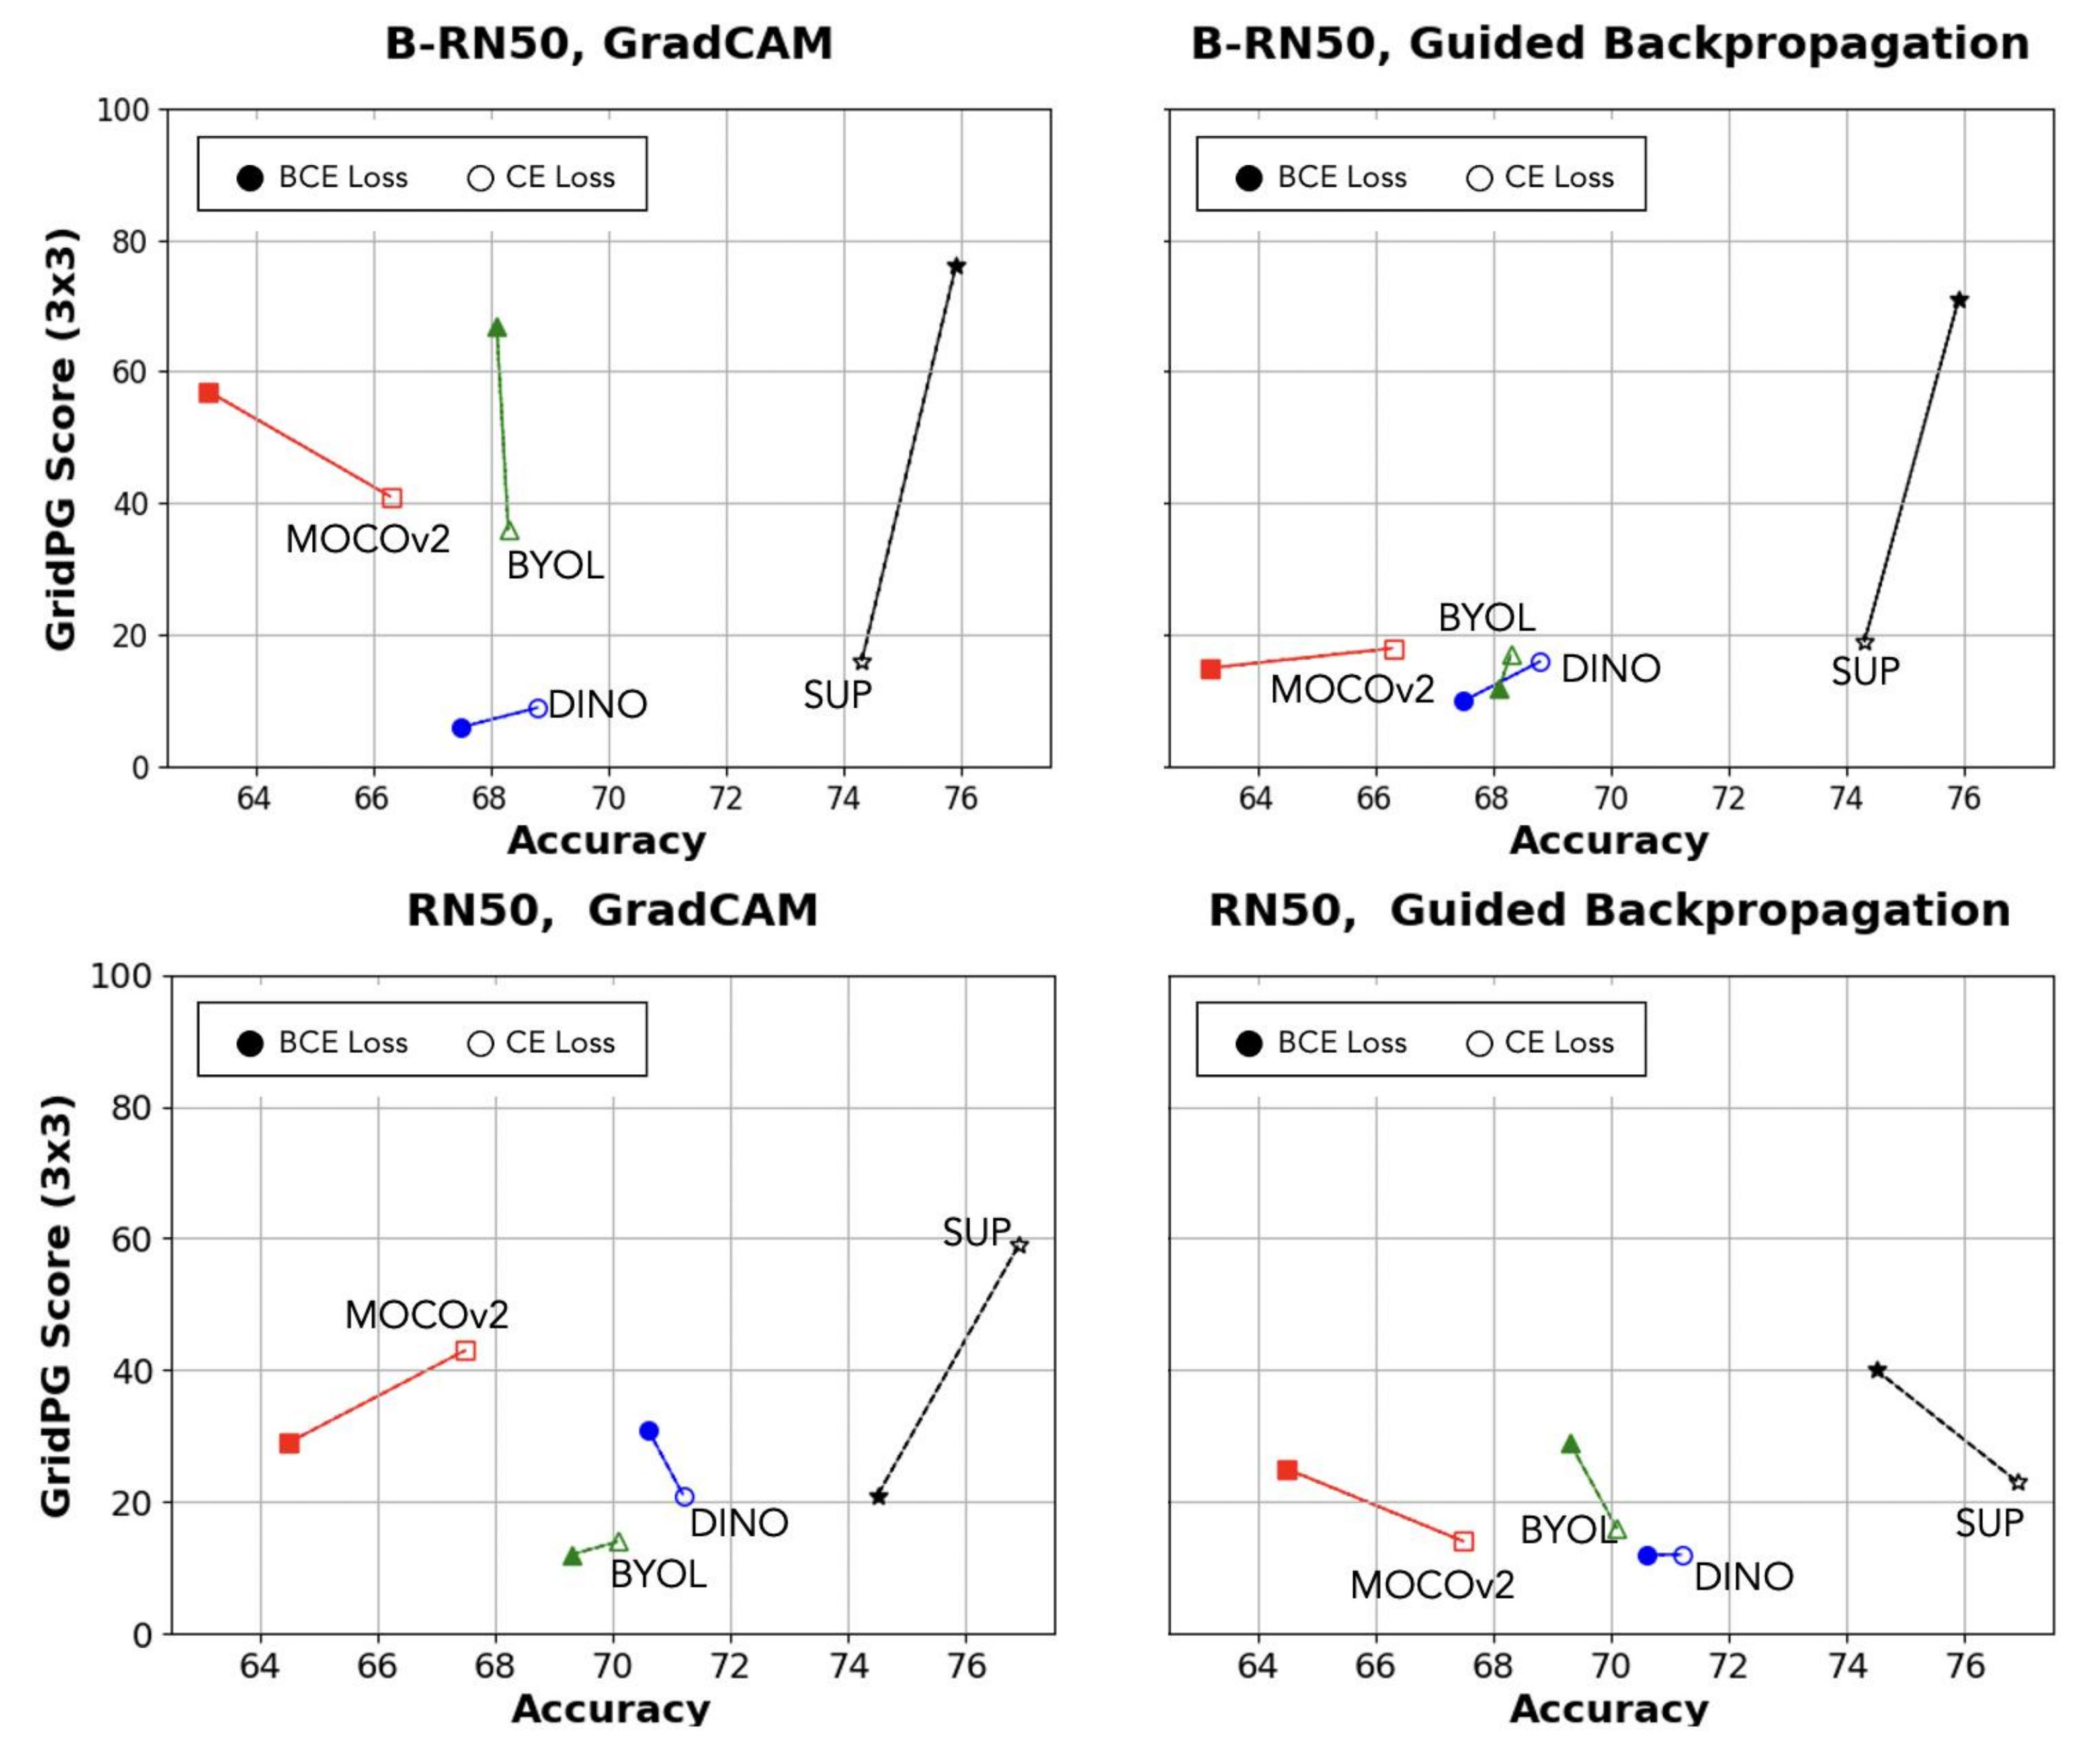}
\end{center}
\vspace{-4mm}
    \caption{{\bf BCE vs.~CE --- Accuracy and \gridpg scores on \imagenet.} \gridpg for GradCAM and GuidedBackpropagation.
    \vspace{-1mm}}
    \label{fig:sup_bce_vs_ce_in1k}
\end{figure*}
