# Supplementary material for: How to Probe: Simple Yet Effective Techniques for Improving Post-hoc Explanations
Source: arXiv:2503.00641 source file (2025-03-01)
Supplement: Supplementary file 2 [file bce_vs_ce_rn50_caltech.tex]

\begin{subfigure}[c]{0.95\linewidth}
\centering
\begin{center}
    \centering
    \includegraphics[width=\linewidth]{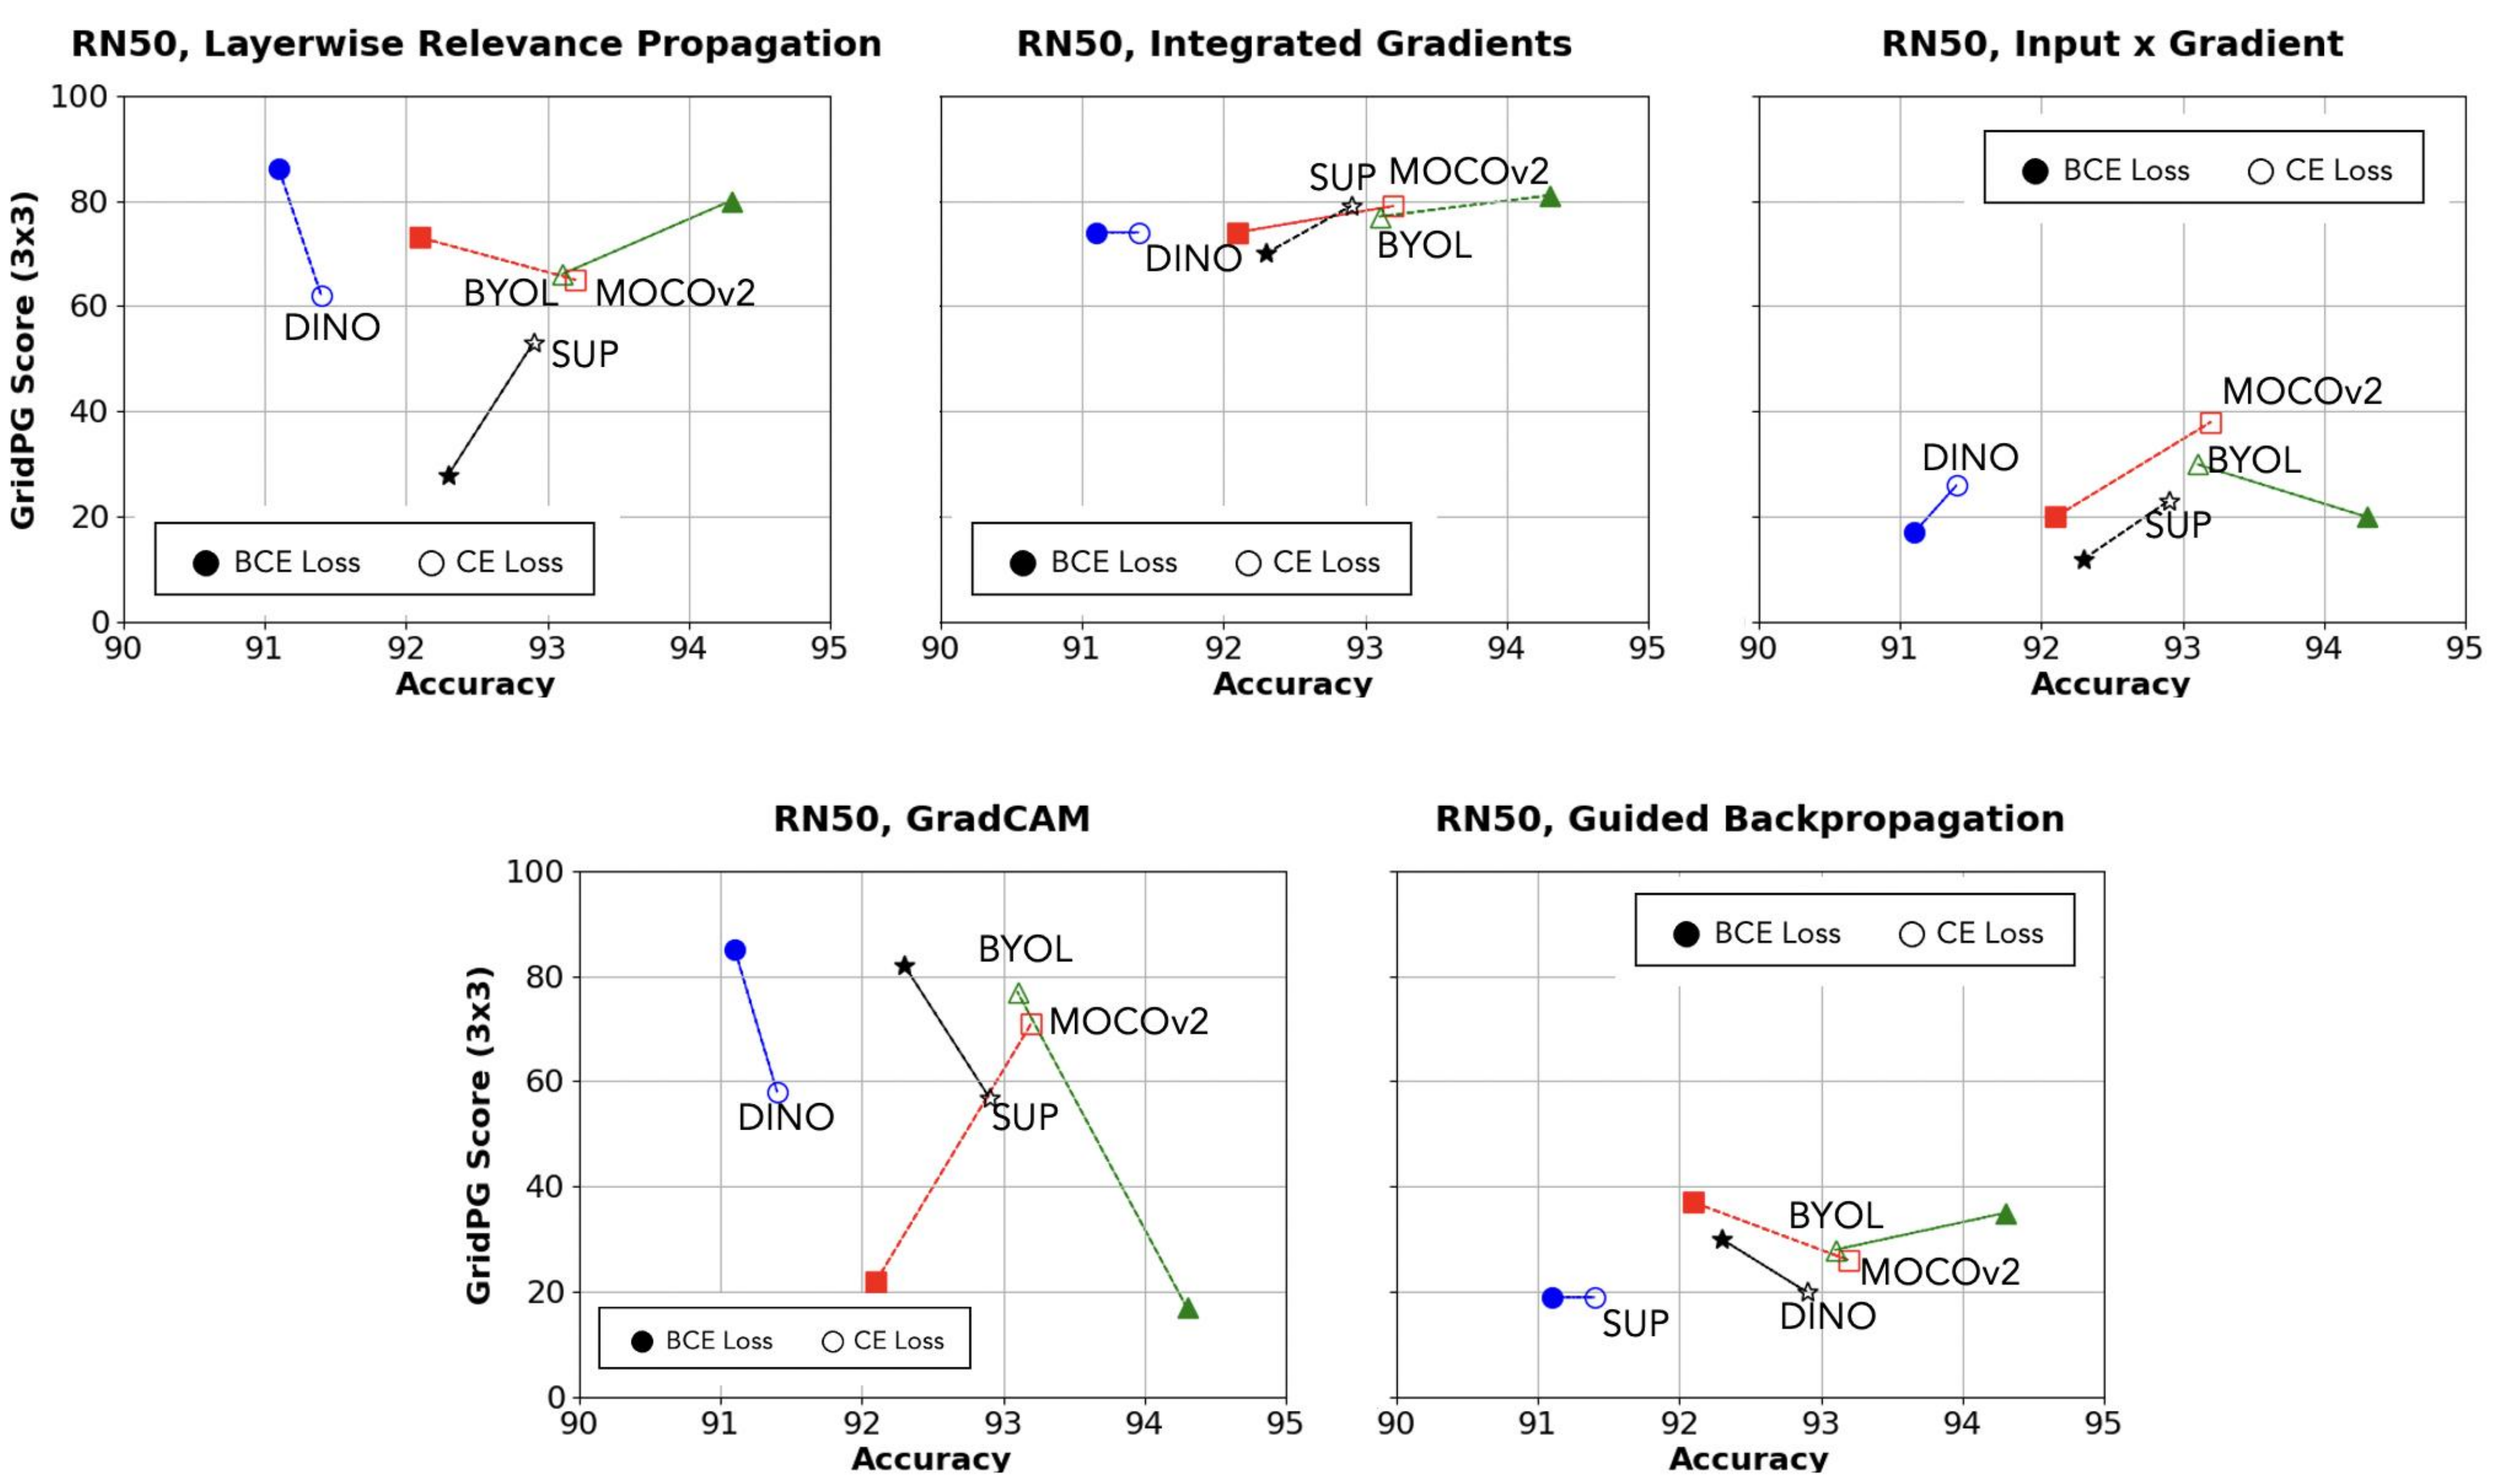}
\end{center}
\vspace{-4mm}
    \caption{
    %\vspace{3mm}
    }
    \label{fig:bce_vs_ce_std_all_caltech}
\end{subfigure}
