# Supplementary material for: How to Probe: Simple Yet Effective Techniques for Improving Post-hoc Explanations
Source: arXiv:2503.00641 source file (2025-03-01)
Supplement: Supplementary file 3 [file mlp_quali_all_v1.tex]

\begin{figure}[h]
  \begin{center}
    \centering
        \includegraphics[width=0.7\linewidth]{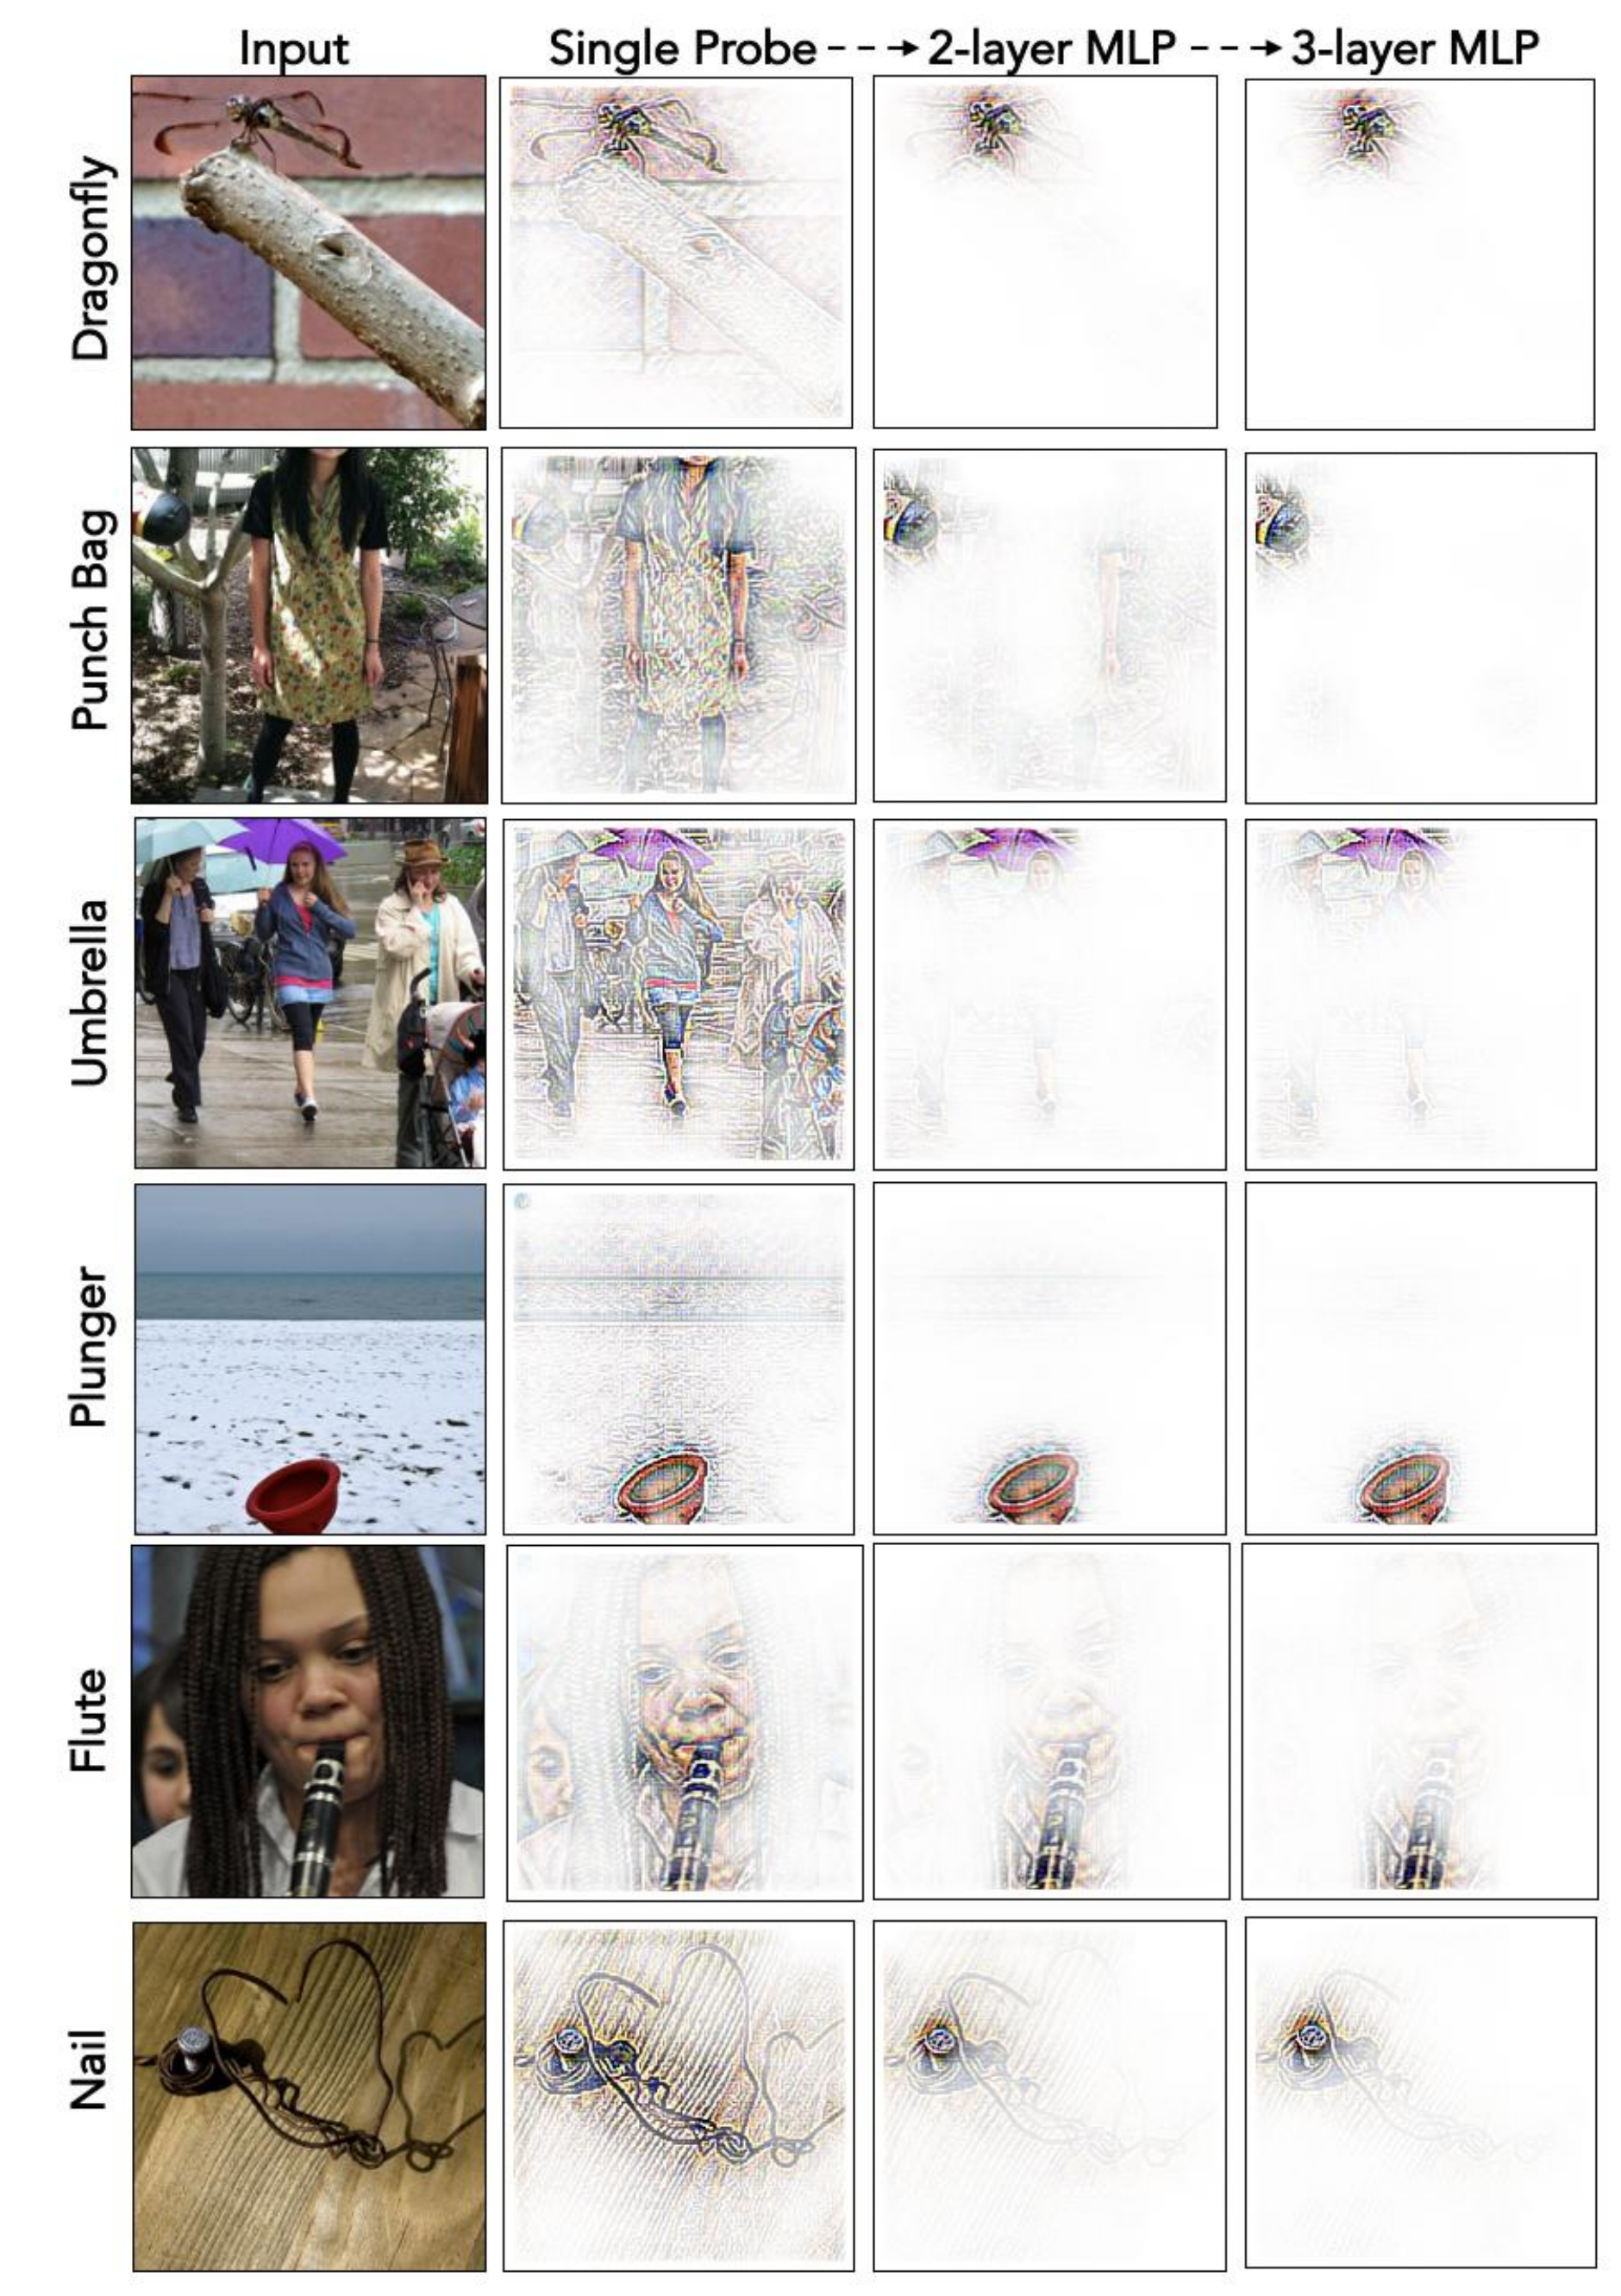}
\end{center}
    \vspace{-4mm}
    \caption{
    \textbf{Qualitative results of MLP probes on \imagenet}. We find that explanations for \bcos MLPs \textbf{(cols. 3+4)} trained on \dino pre-trained features exhibit better localization than a single linear probe (\textbf{col. 2}). This can also be seen for \byol and \moco.
    \vspace{-1mm}
    \label{fig:mlp_qual_dino}
    }

\end{figure}

\begin{figure}
  \begin{center}
    \centering
        \includegraphics[width=0.75\linewidth]{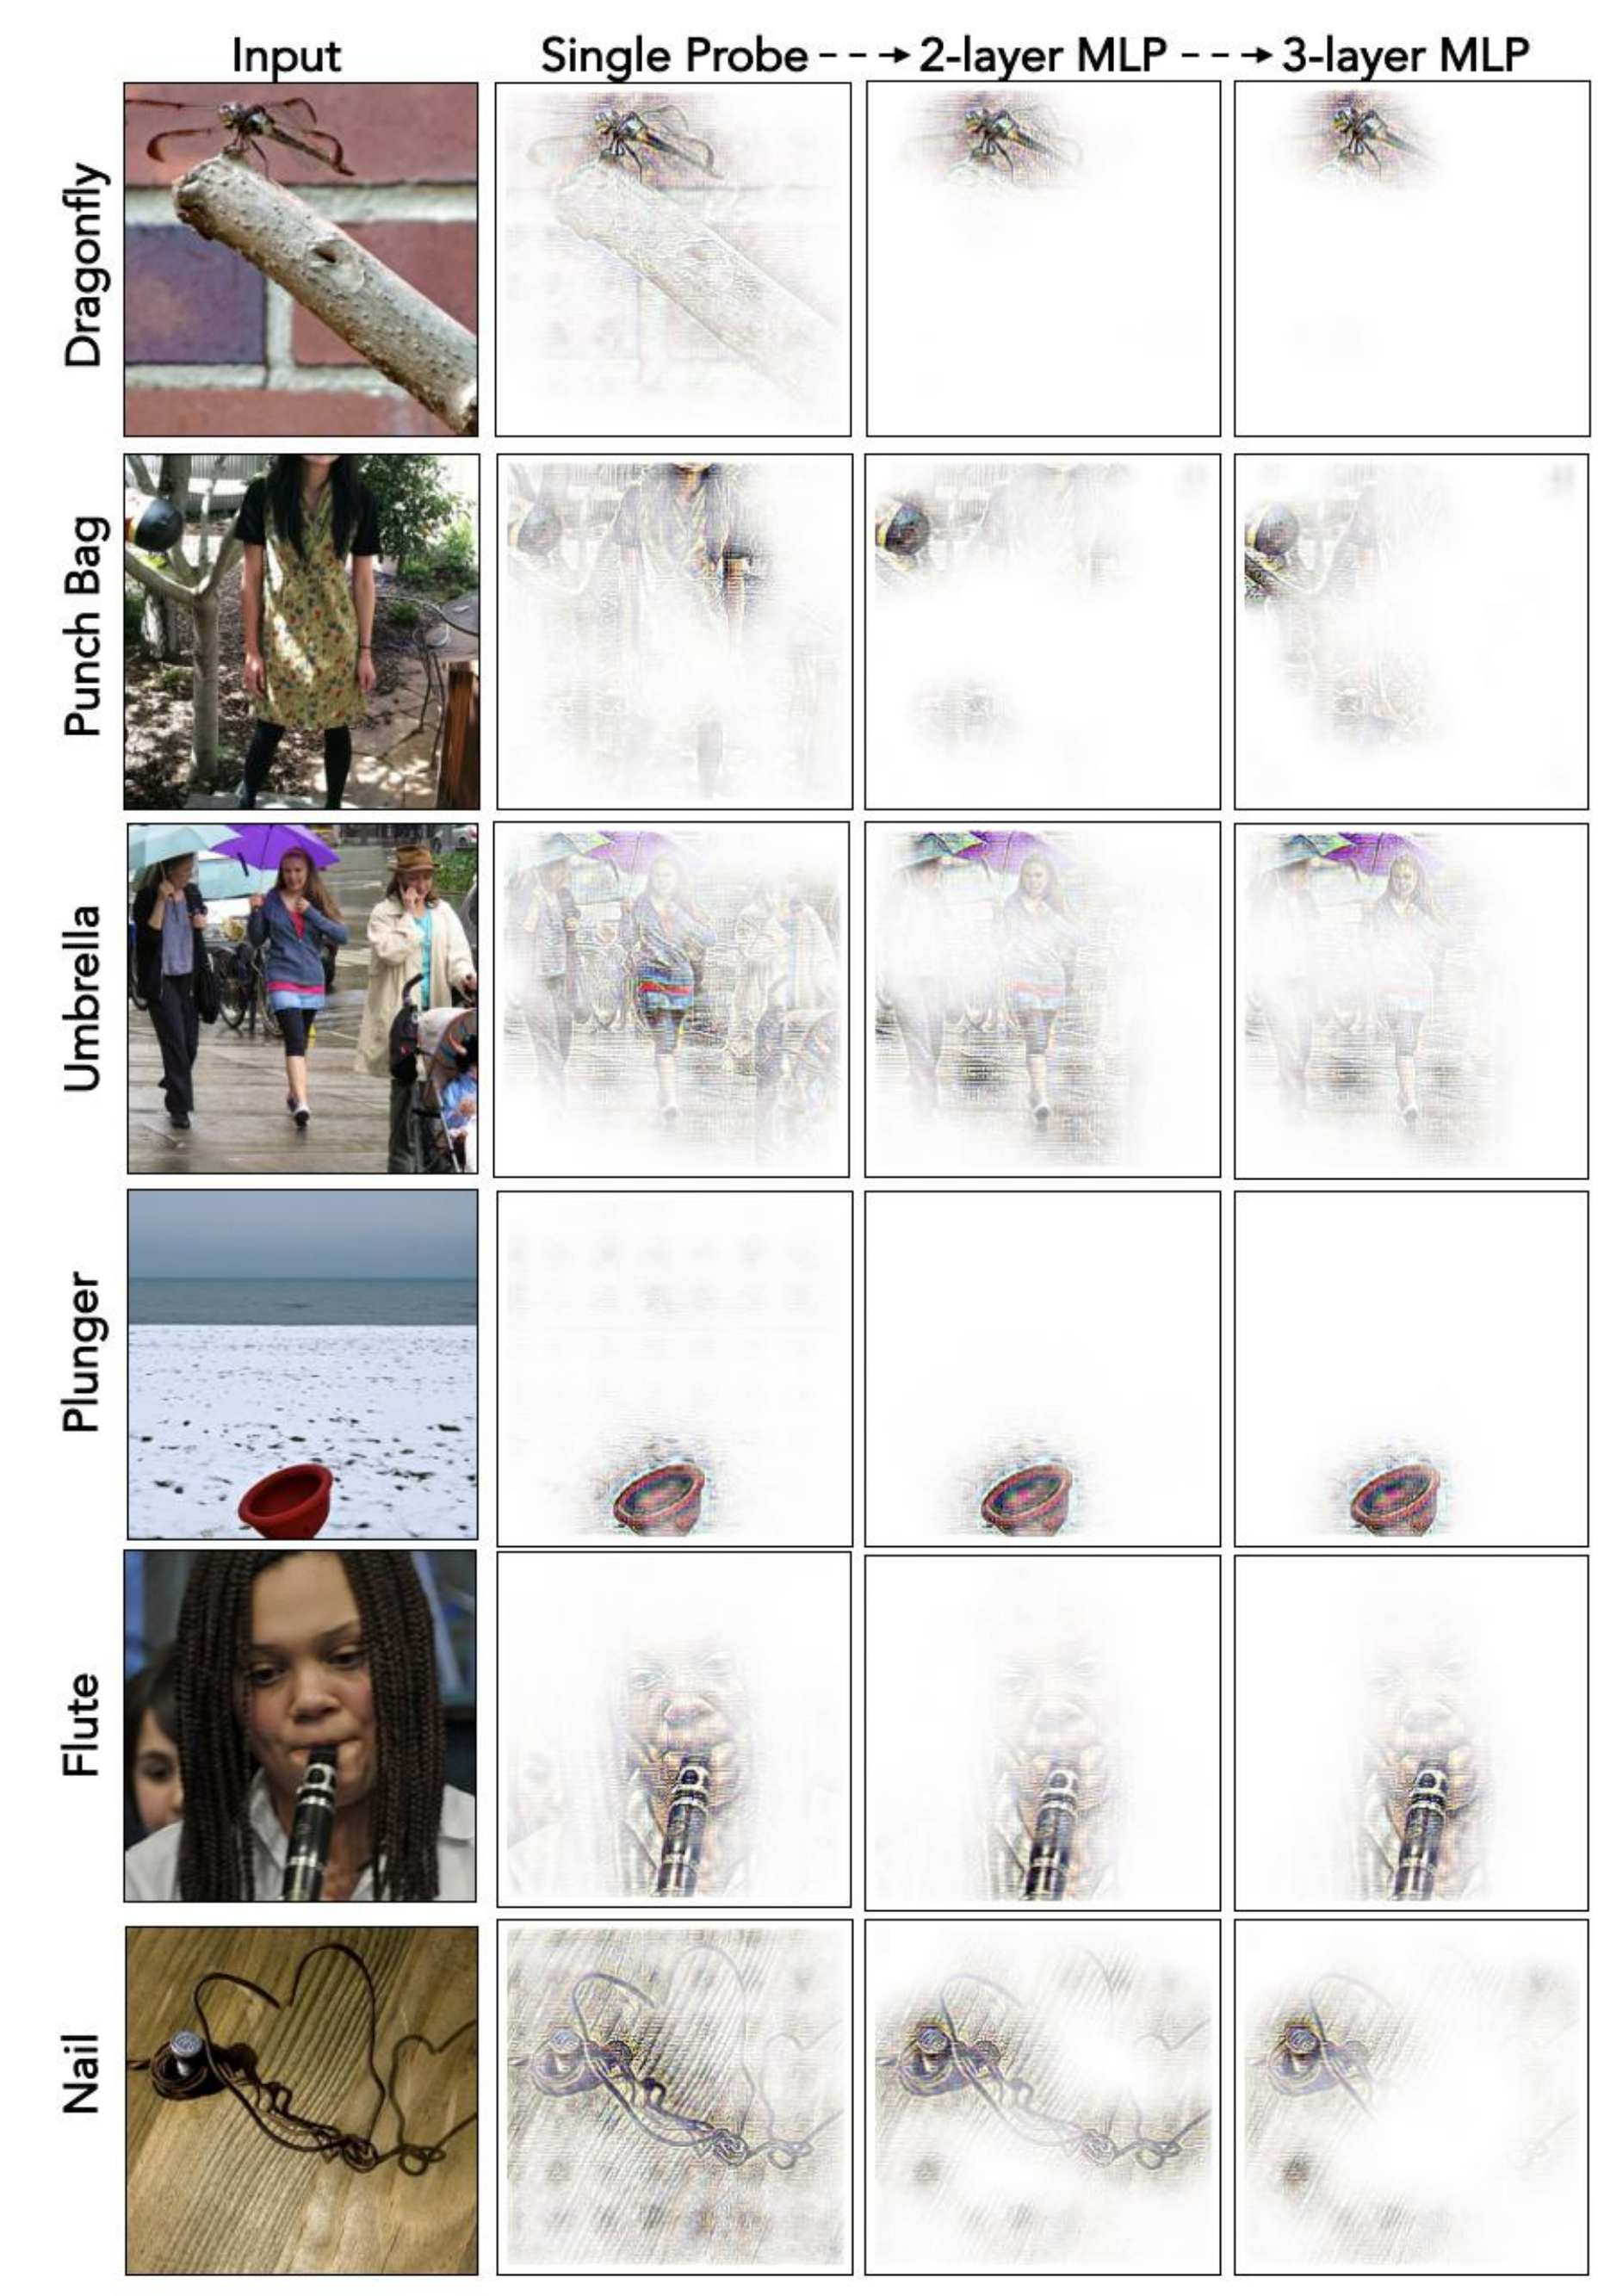}
\end{center}
    \vspace{-4mm}
    \caption{
    \textbf{Qualitative results of MLP probes on \imagenet}. Similar to \cref{fig:mlp_qual_dino}, we find that explanations for \bcos MLPs \textbf{(cols. 3+4)} trained on \byol pre-trained features exhibit better localization than a single linear probe (\textbf{col. 2}). 
    \vspace{-1mm}
    \label{fig:mlp_qual_byol}
    }

\end{figure}

\begin{figure}
  \begin{center}
    \centering
        \includegraphics[width=0.75\linewidth]{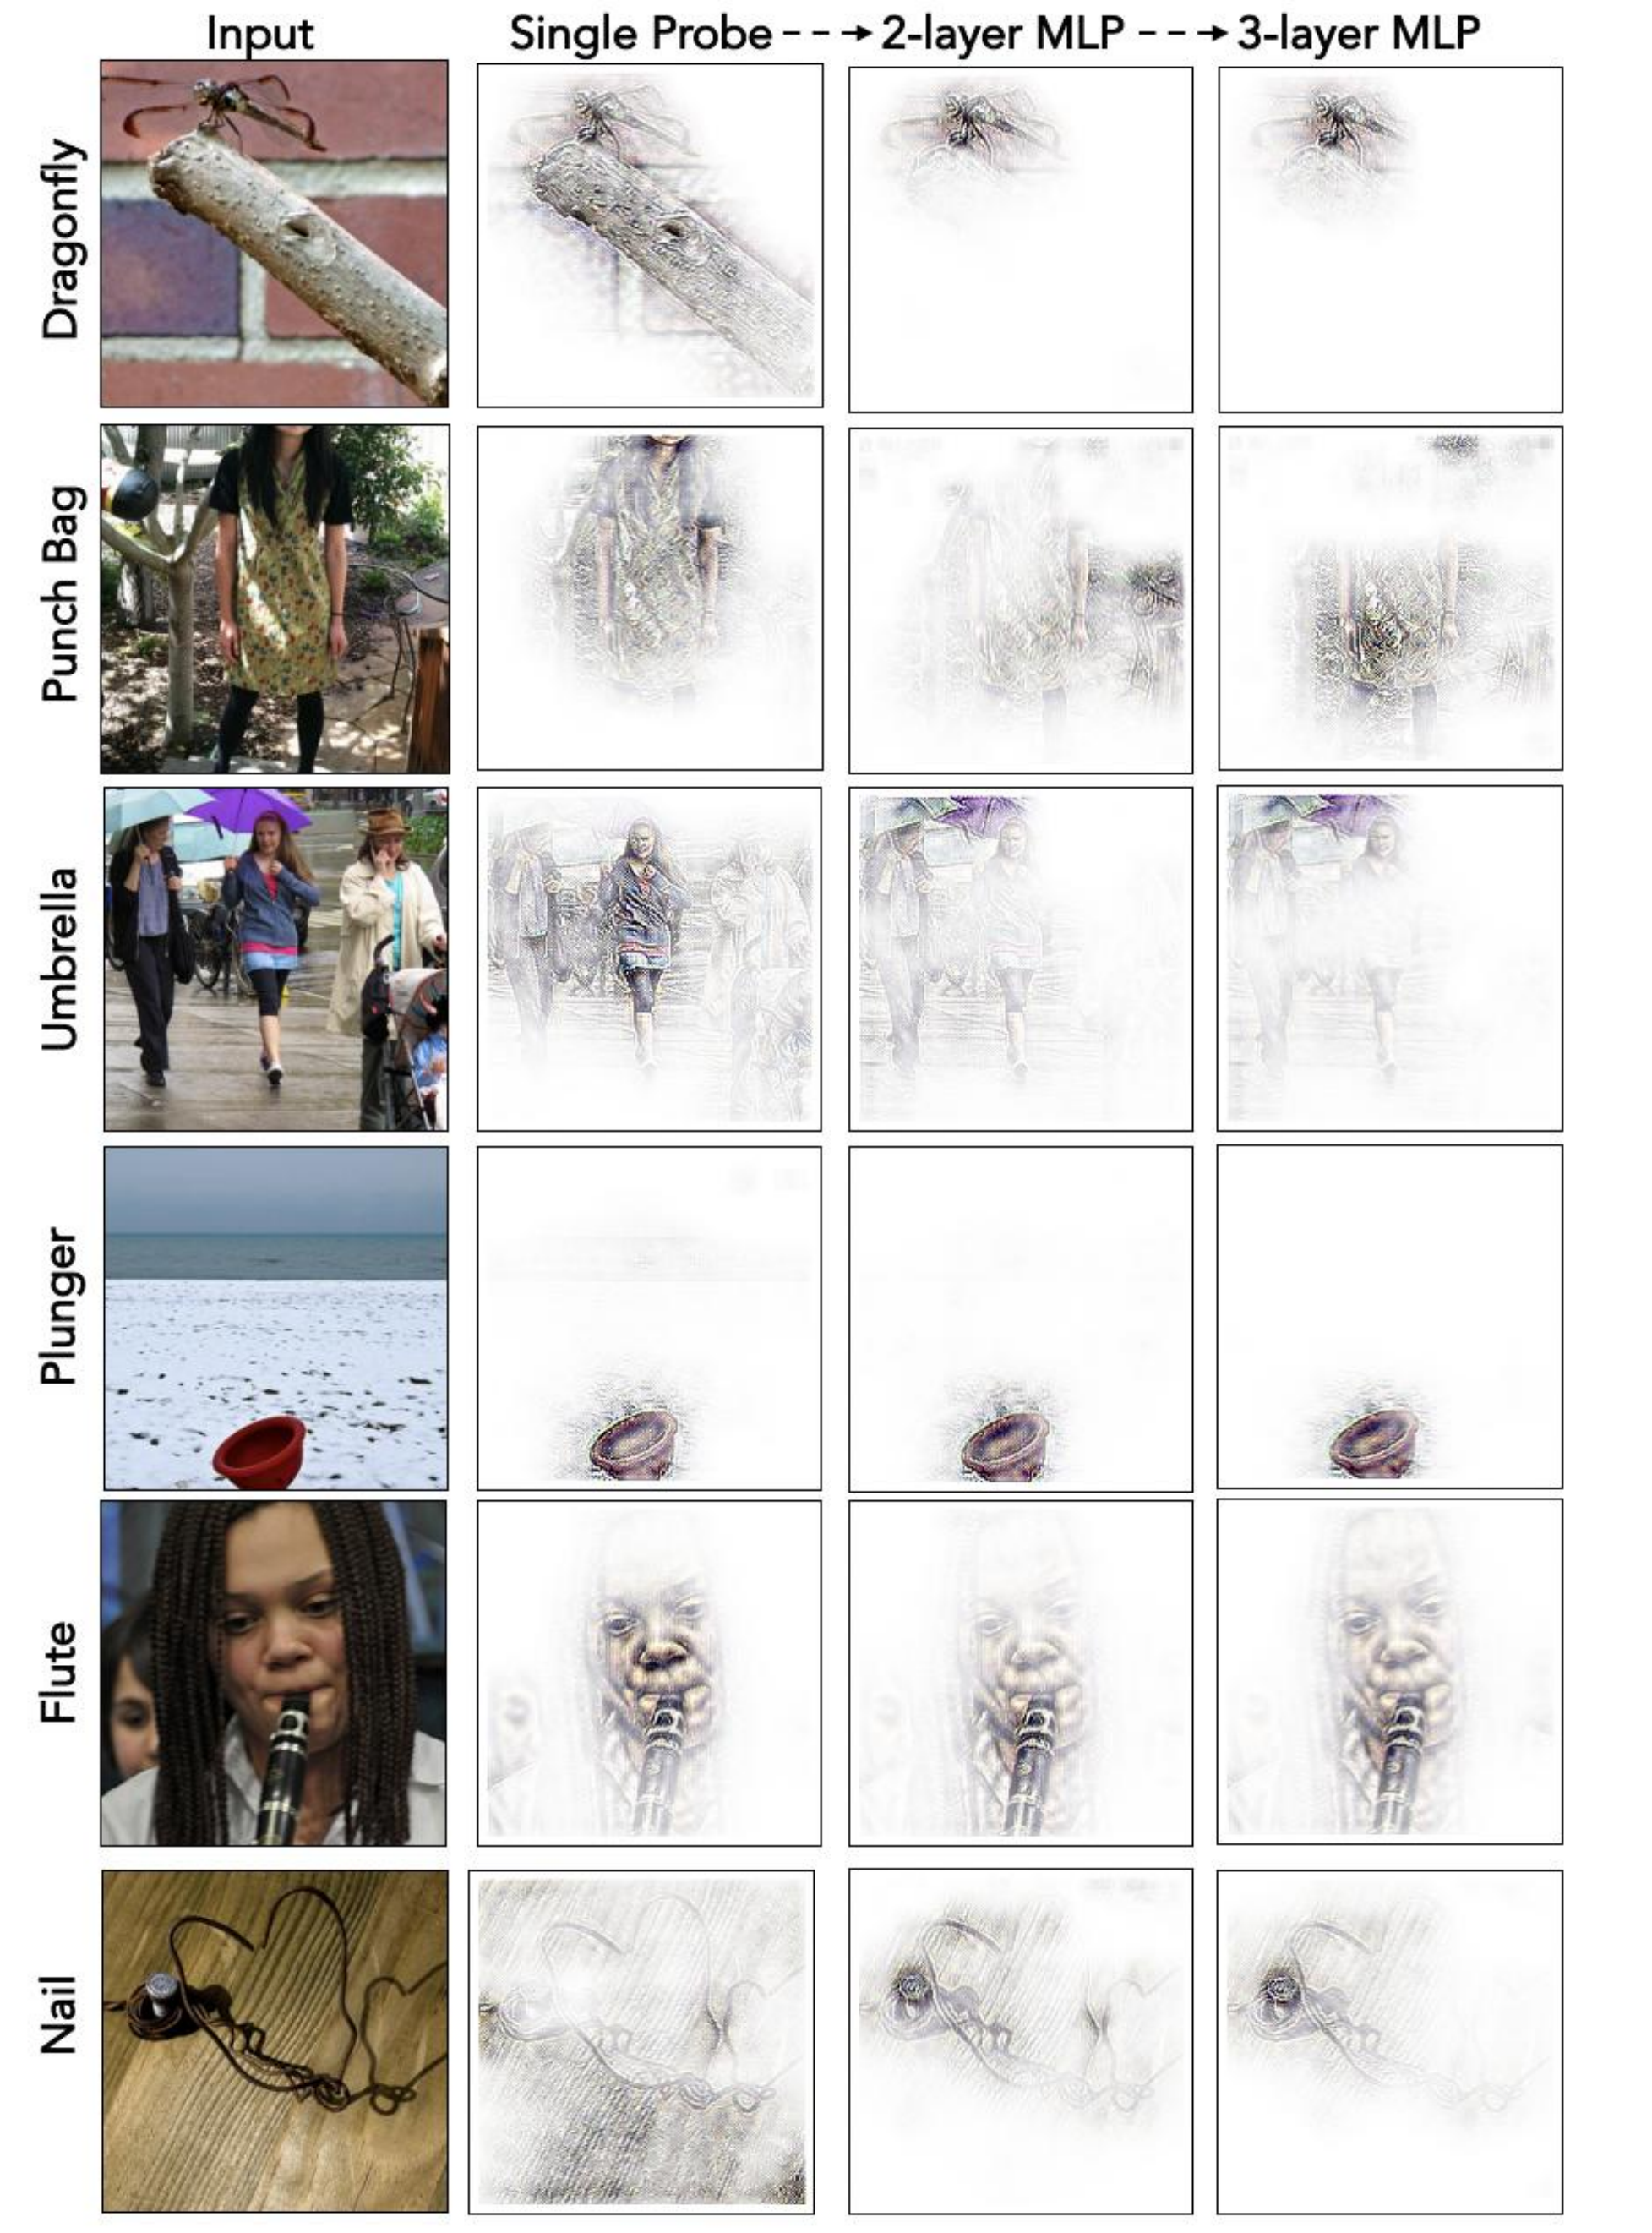}
\end{center}
    \vspace{-4mm}
    \caption{
    \textbf{Qualitative results of MLP probes on \imagenet}. Similar to \cref{fig:mlp_qual_dino}, \ref{fig:mlp_qual_moco} we find explanations for \bcos MLPs \textbf{(cols. 3+4)} trained on \moco pre-trained features to exhibit better localization than a single linear probe (\textbf{col. 2}). 
    \vspace{-1mm}
   \label{fig:mlp_qual_moco}
   }
\end{figure}
