# Supplementary material for: How to Probe: Simple Yet Effective Techniques for Improving Post-hoc Explanations
Source: arXiv:2503.00641 source file (2025-03-01)
Supplement: Supplementary file 4 [file qual_all_v1.tex]

\begin{figure}[h]
  \begin{center}
    \centering
        \includegraphics[width=0.65\linewidth]{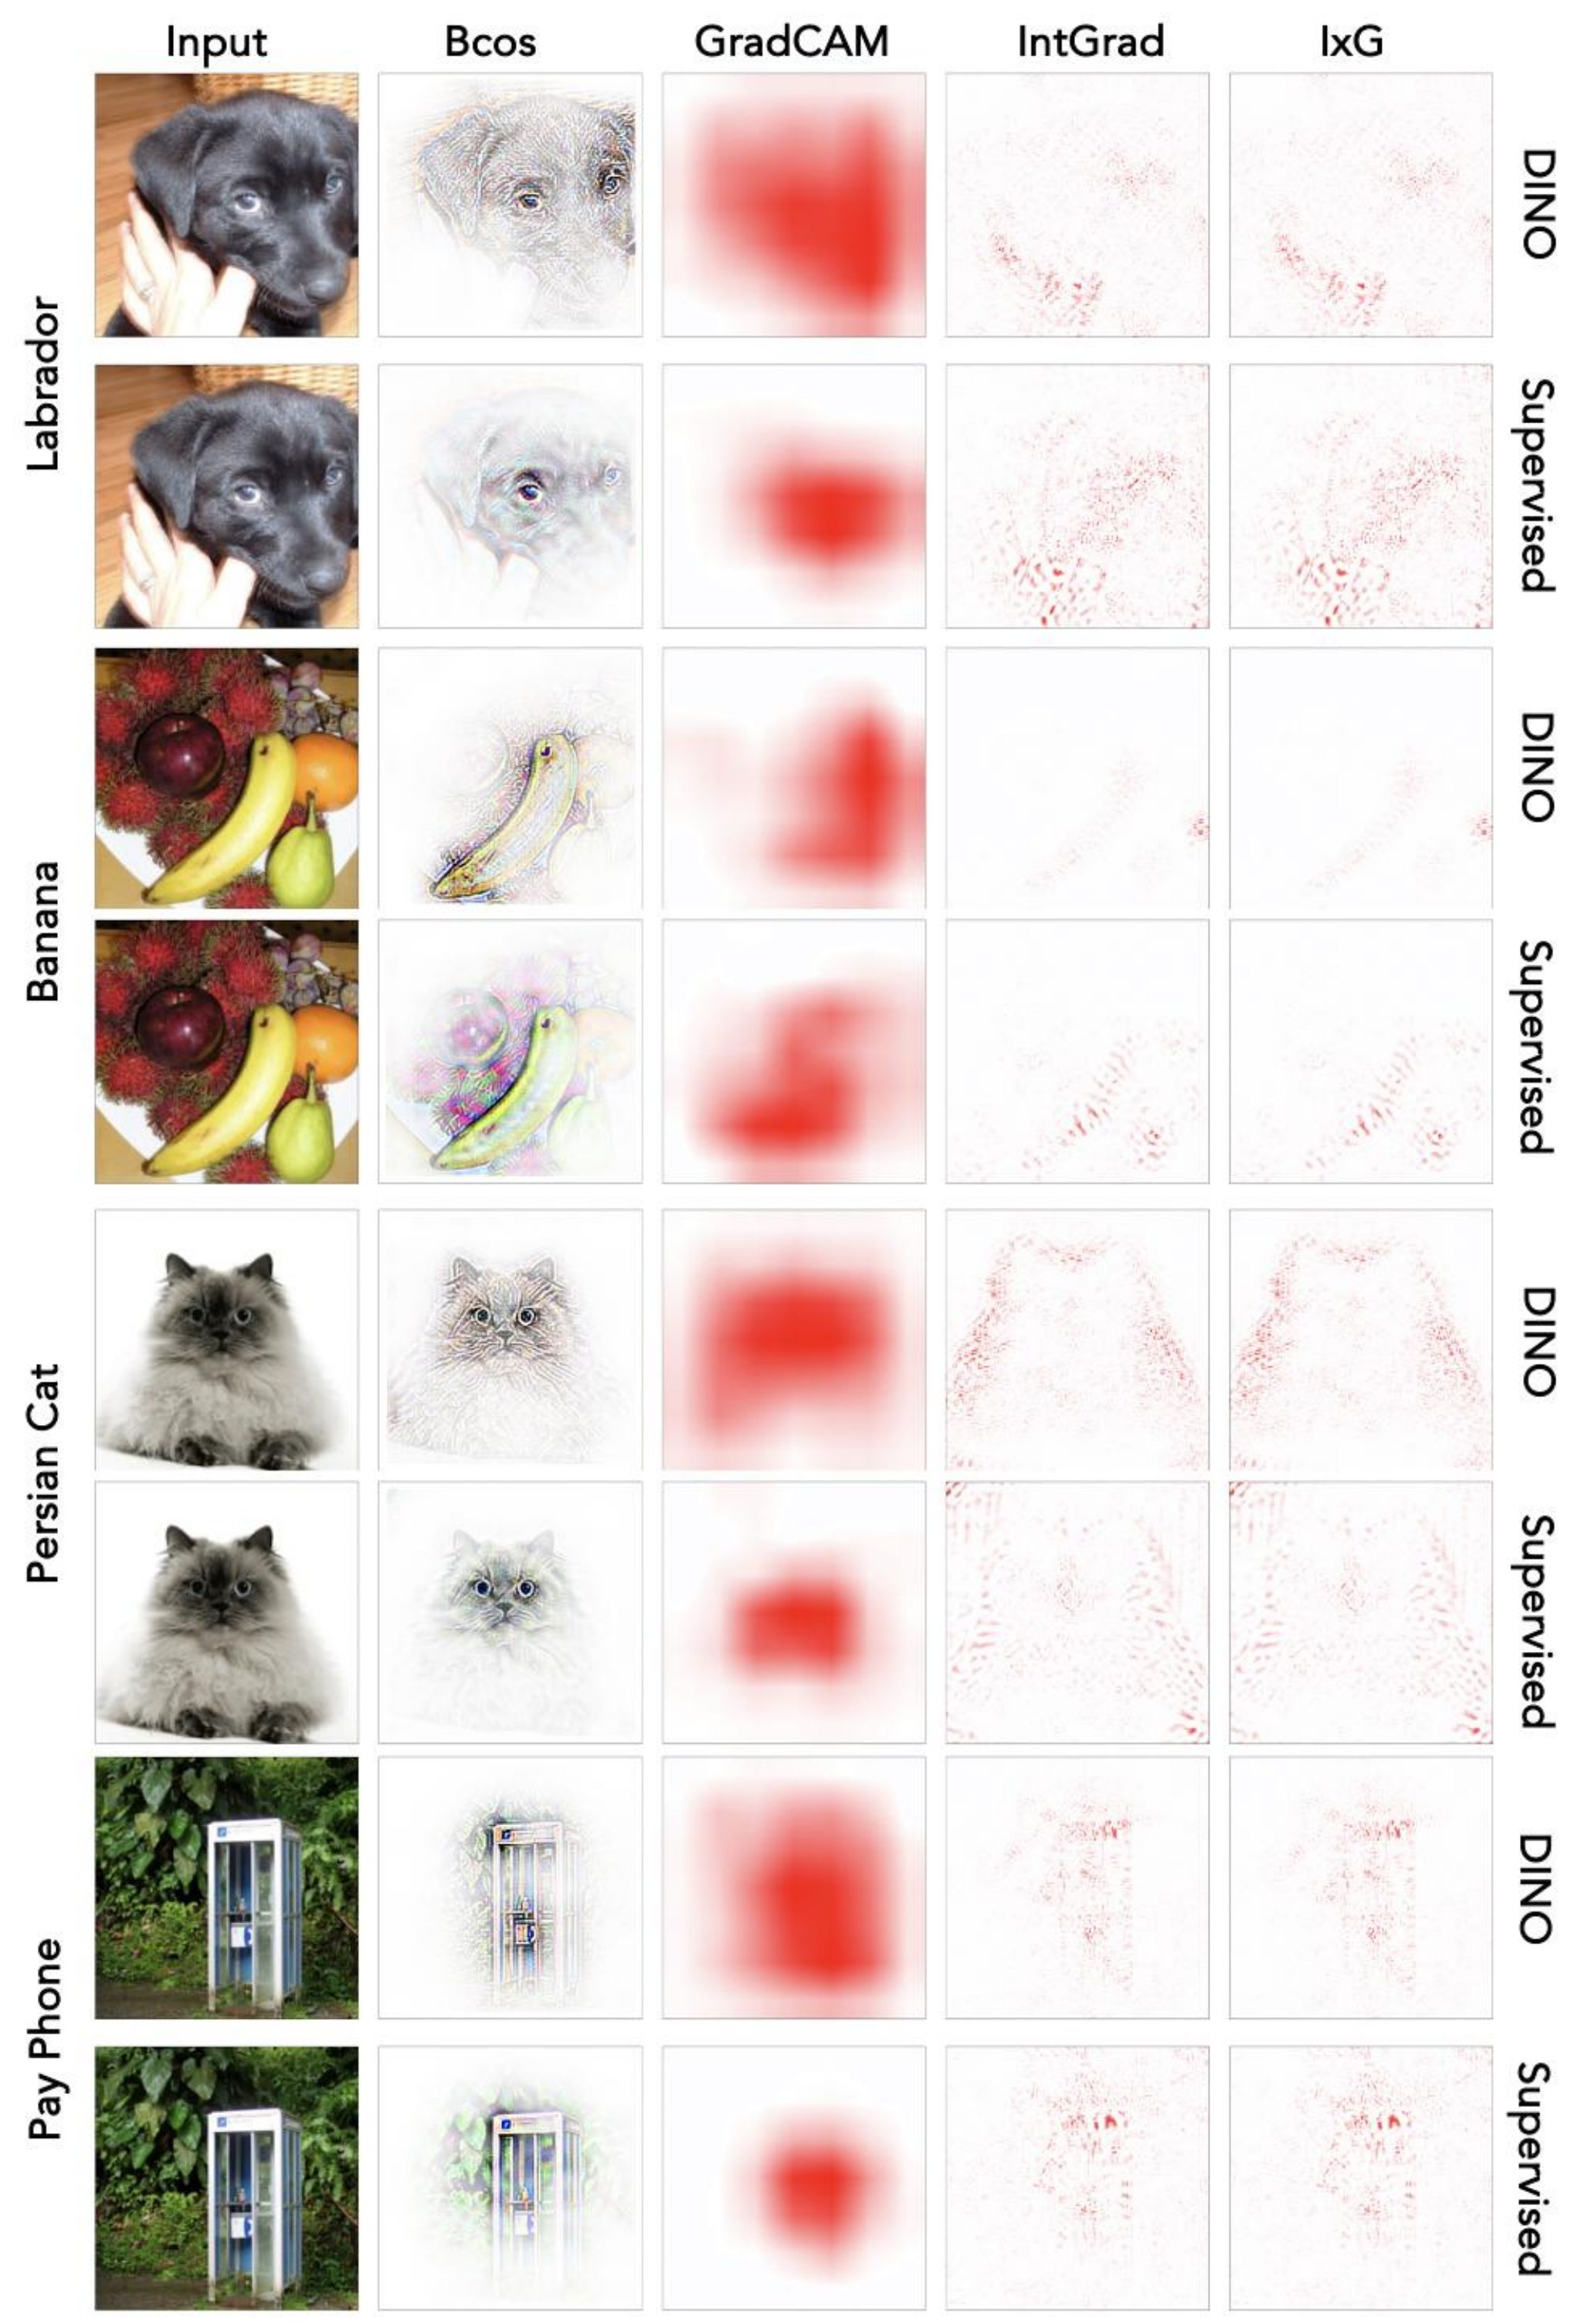}
\end{center}
    \vspace{-4mm}
    \caption
    {
    Qualitative results for different explanation methods for \textbf{\dino} and supervised \bcos models.
    \vspace{-1mm}
    }
   \label{fig:qual_bcos_dino}
\end{figure}

\begin{figure}[h]
  \begin{center}
    \centering
        \includegraphics[width=0.85\linewidth]{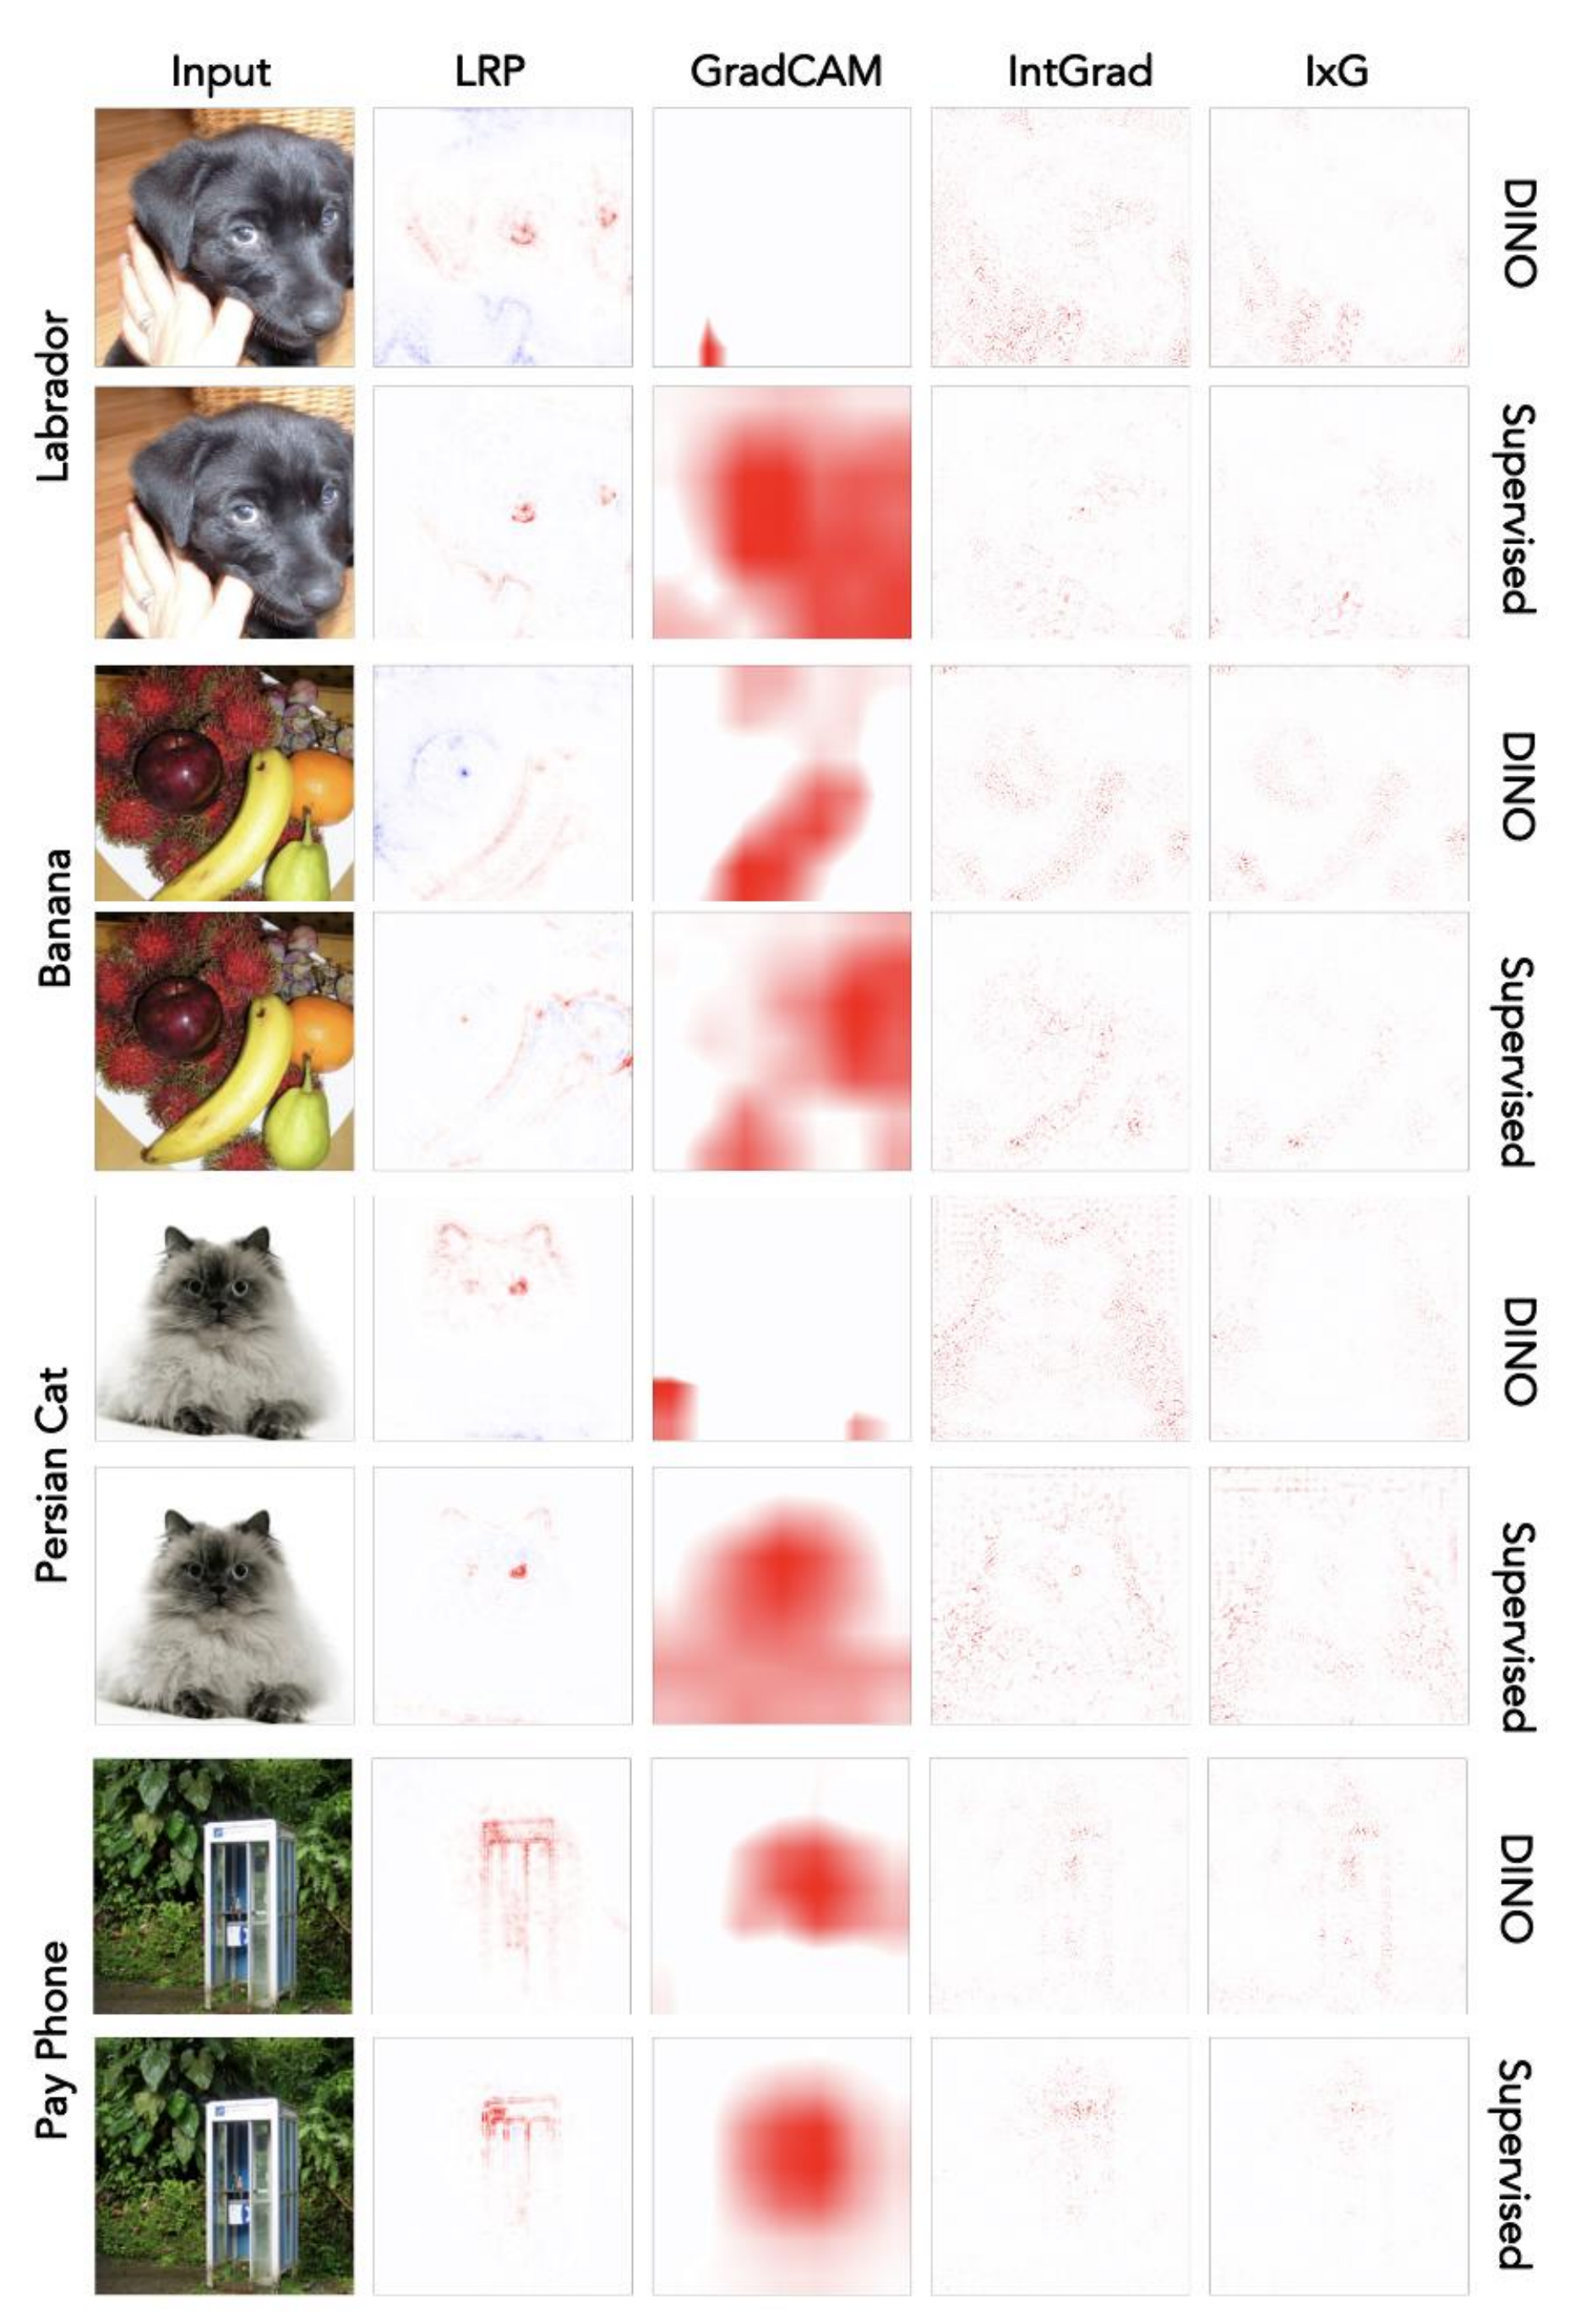}
\end{center}
    \vspace{-4mm}
    \caption
    {
        Qualitative results for different explanation methods for \textbf{\dino} and supervised conventional models.
    \vspace{-1mm}
    }
   \label{fig:qual_std_dino}
\end{figure}

\begin{figure}[h]
  \begin{center}
    \centering
        \includegraphics[width=0.85\linewidth]{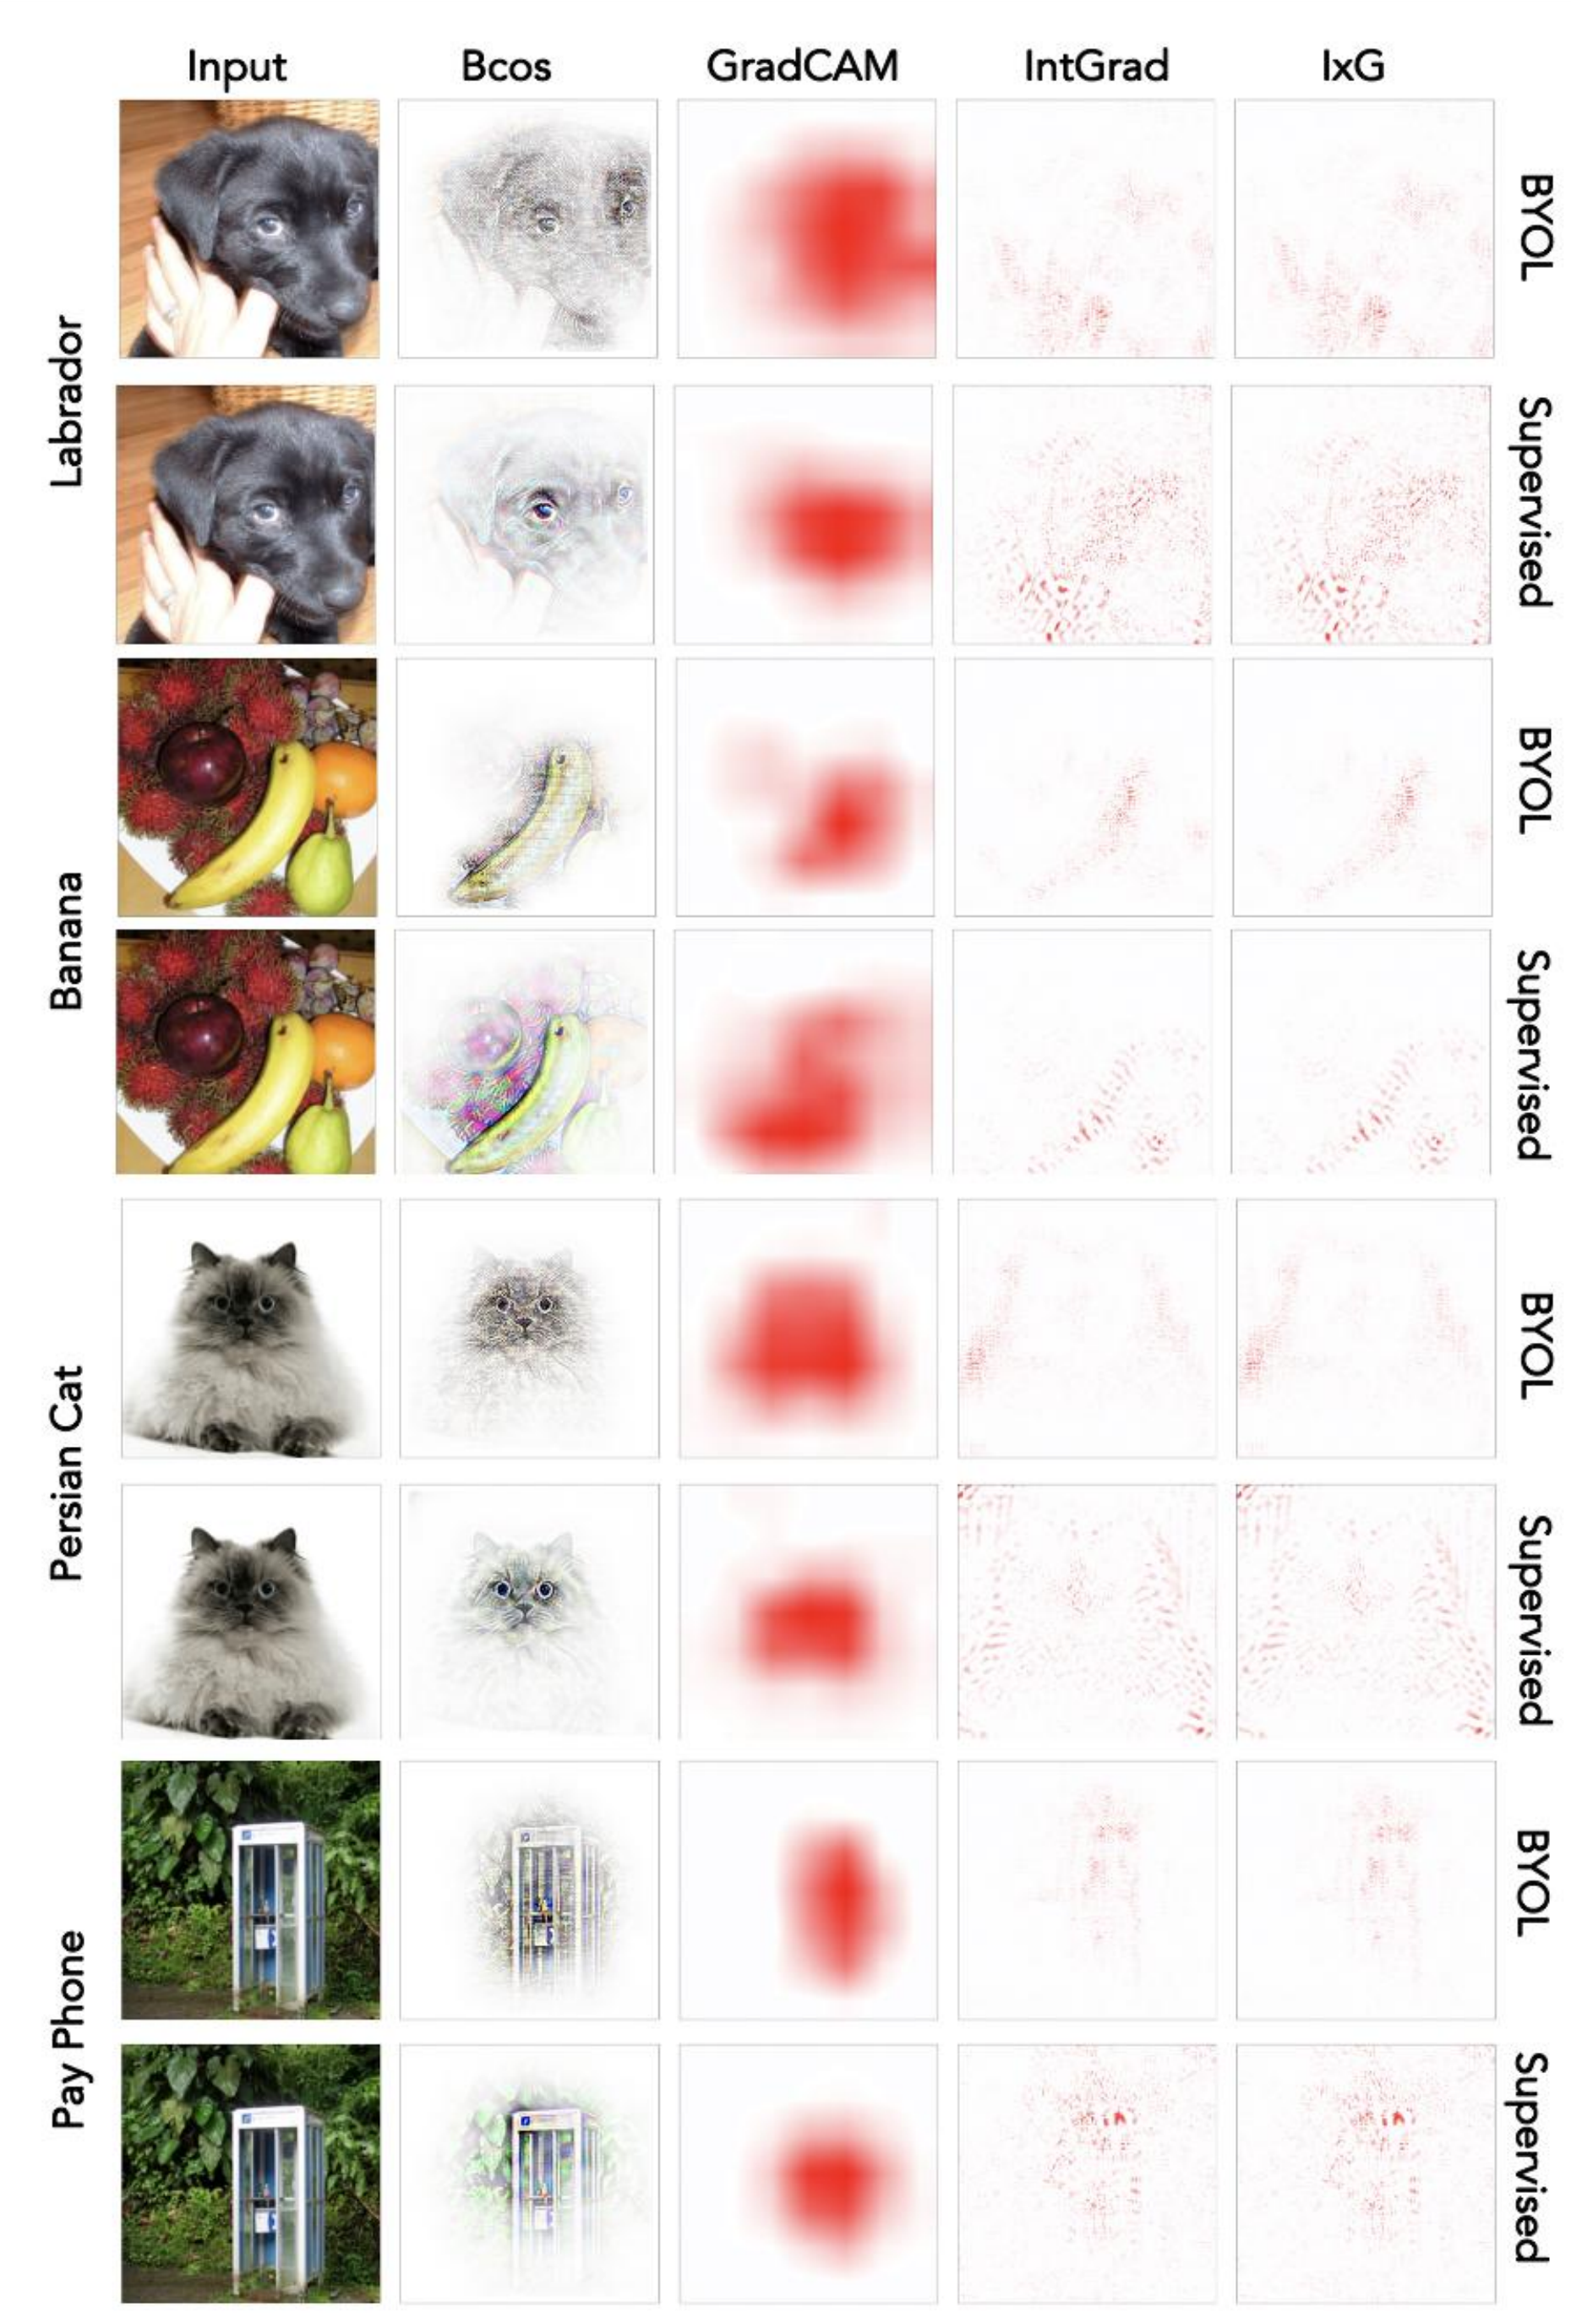}
\end{center}
    \vspace{-4mm}
    \caption
    {    Qualitative results for different explanation methods for \textbf{\byol} and supervised \bcos models.
    \vspace{-1mm}
    }
   \label{fig:qual_bcos_byol}
\end{figure}

\begin{figure}
  \begin{center}
    \centering
        \includegraphics[width=0.85\linewidth]{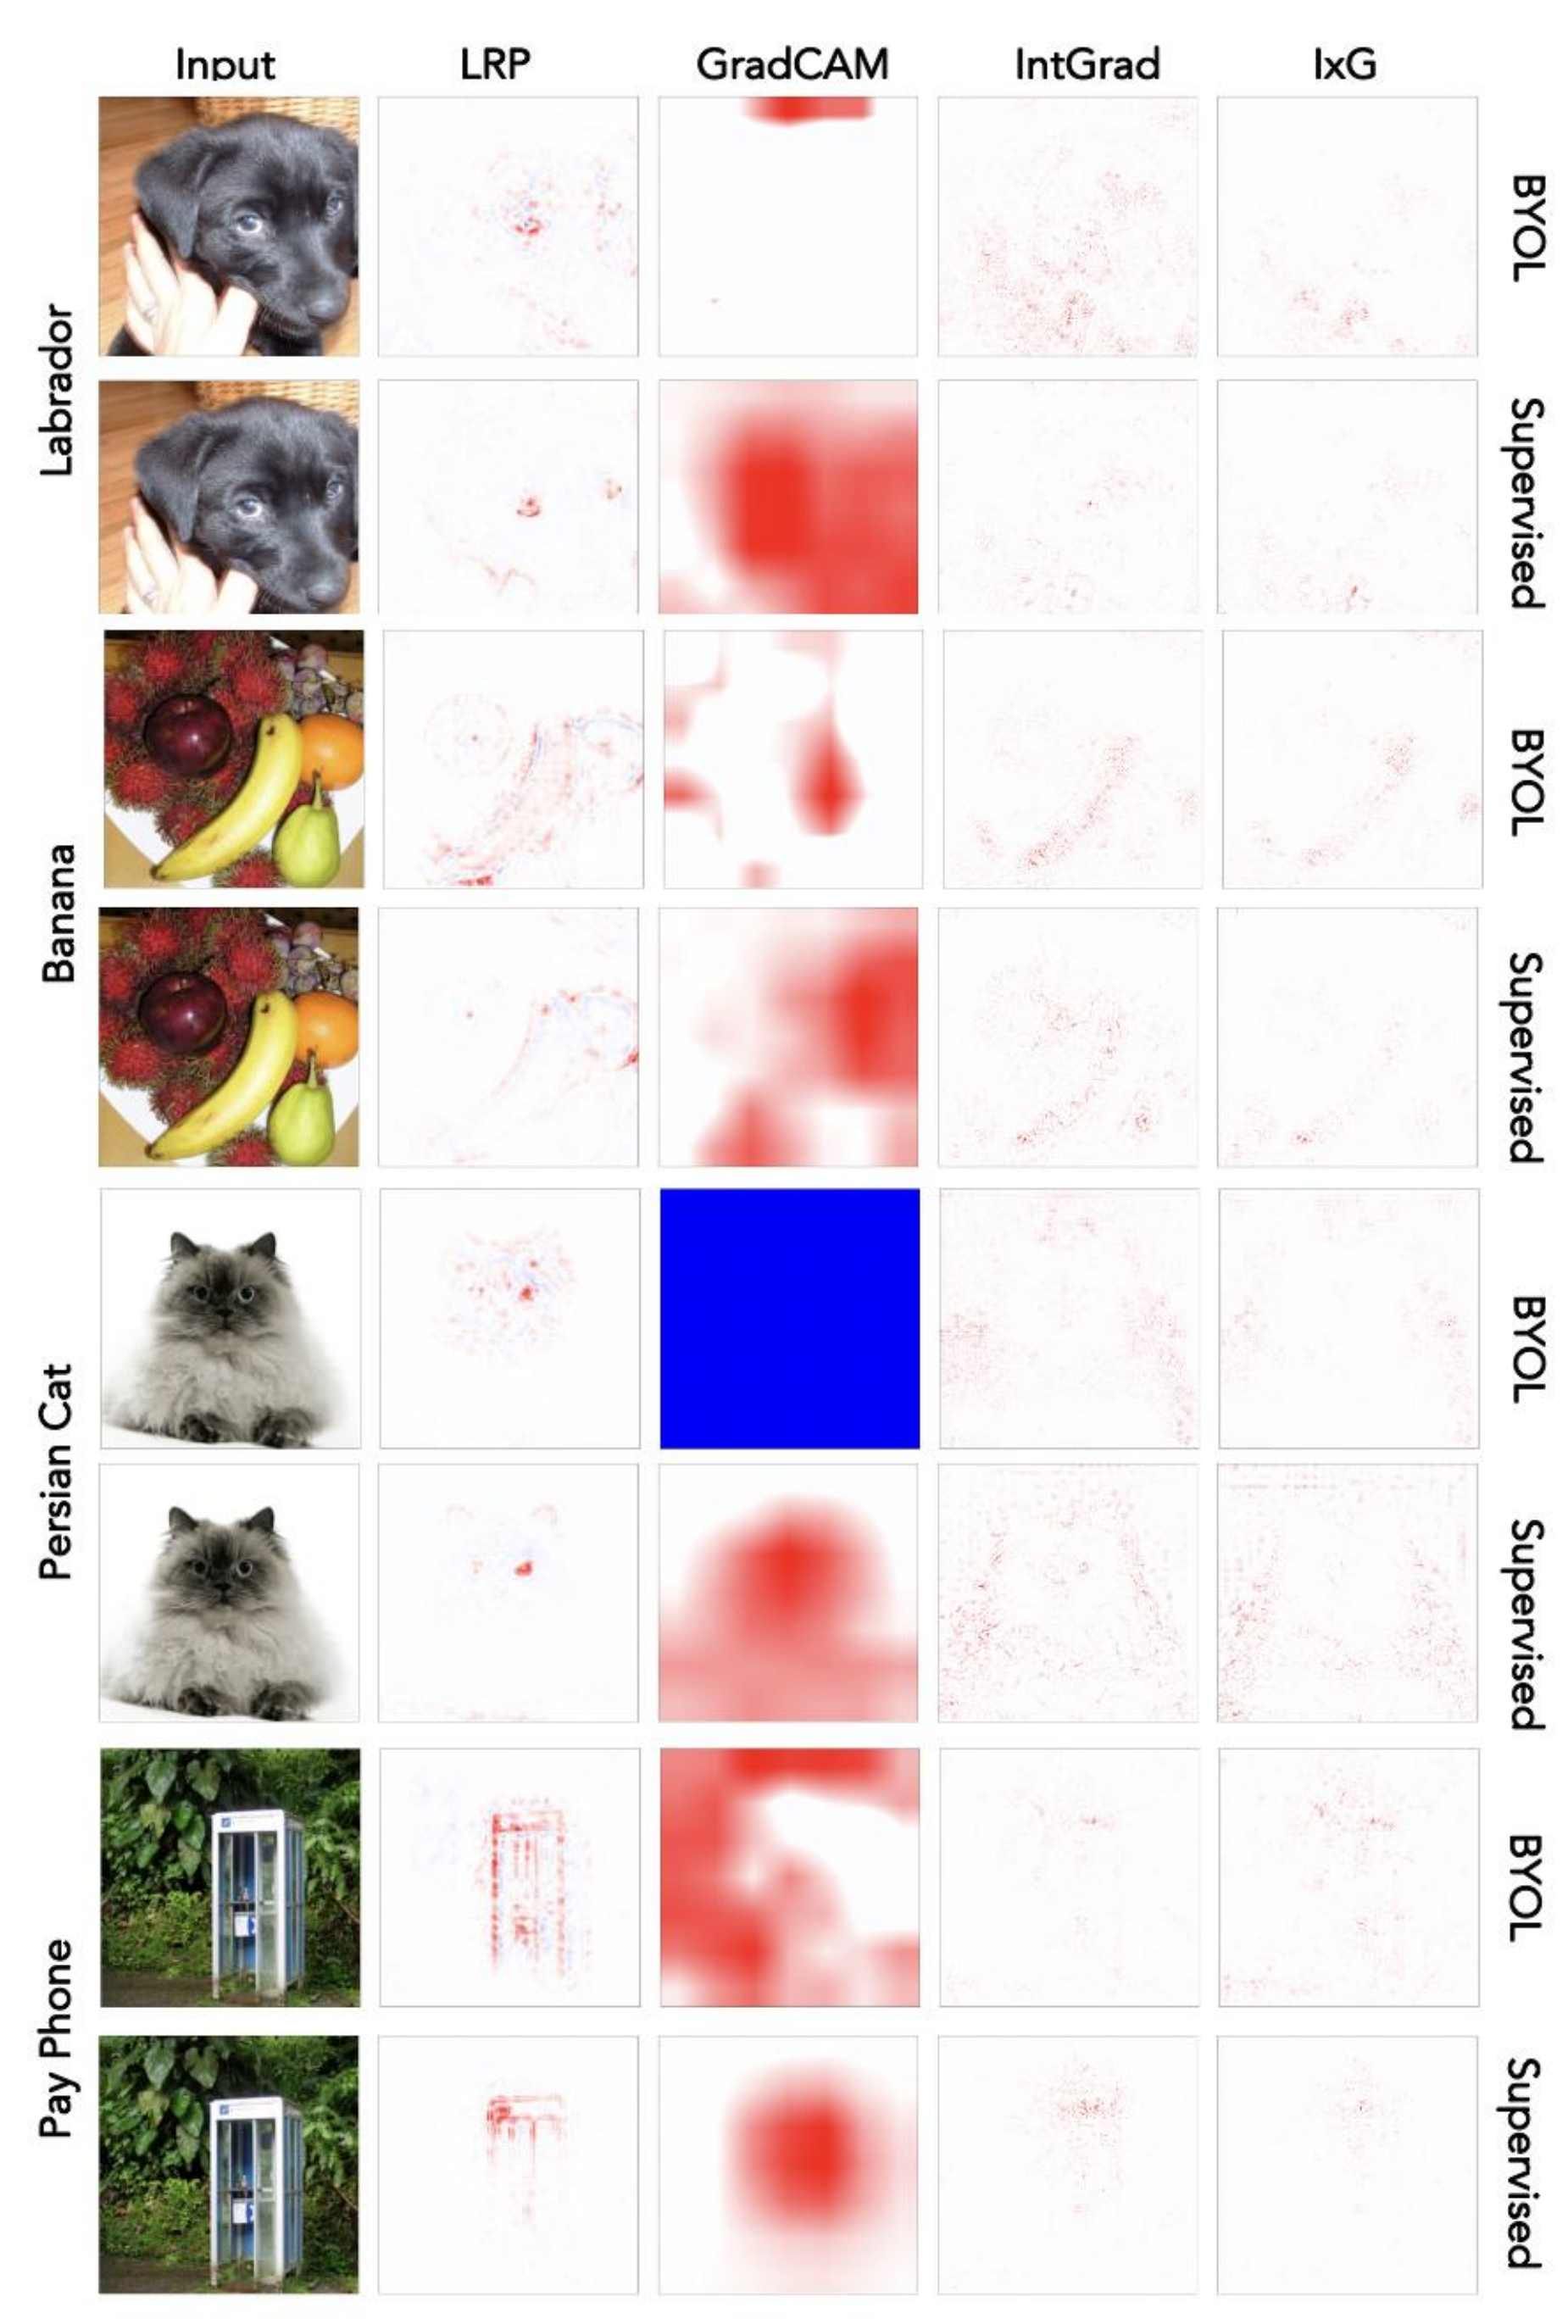}
\end{center}
    \vspace{-4mm}
    \caption
    { Qualitative results for different explanation methods for \textbf{\byol} and supervised conventional models.
    \vspace{-1mm}
    }
   \label{fig:qual_std_byol}
\end{figure}

\begin{figure}
  \begin{center}
    \centering
        \includegraphics[width=0.85\linewidth]{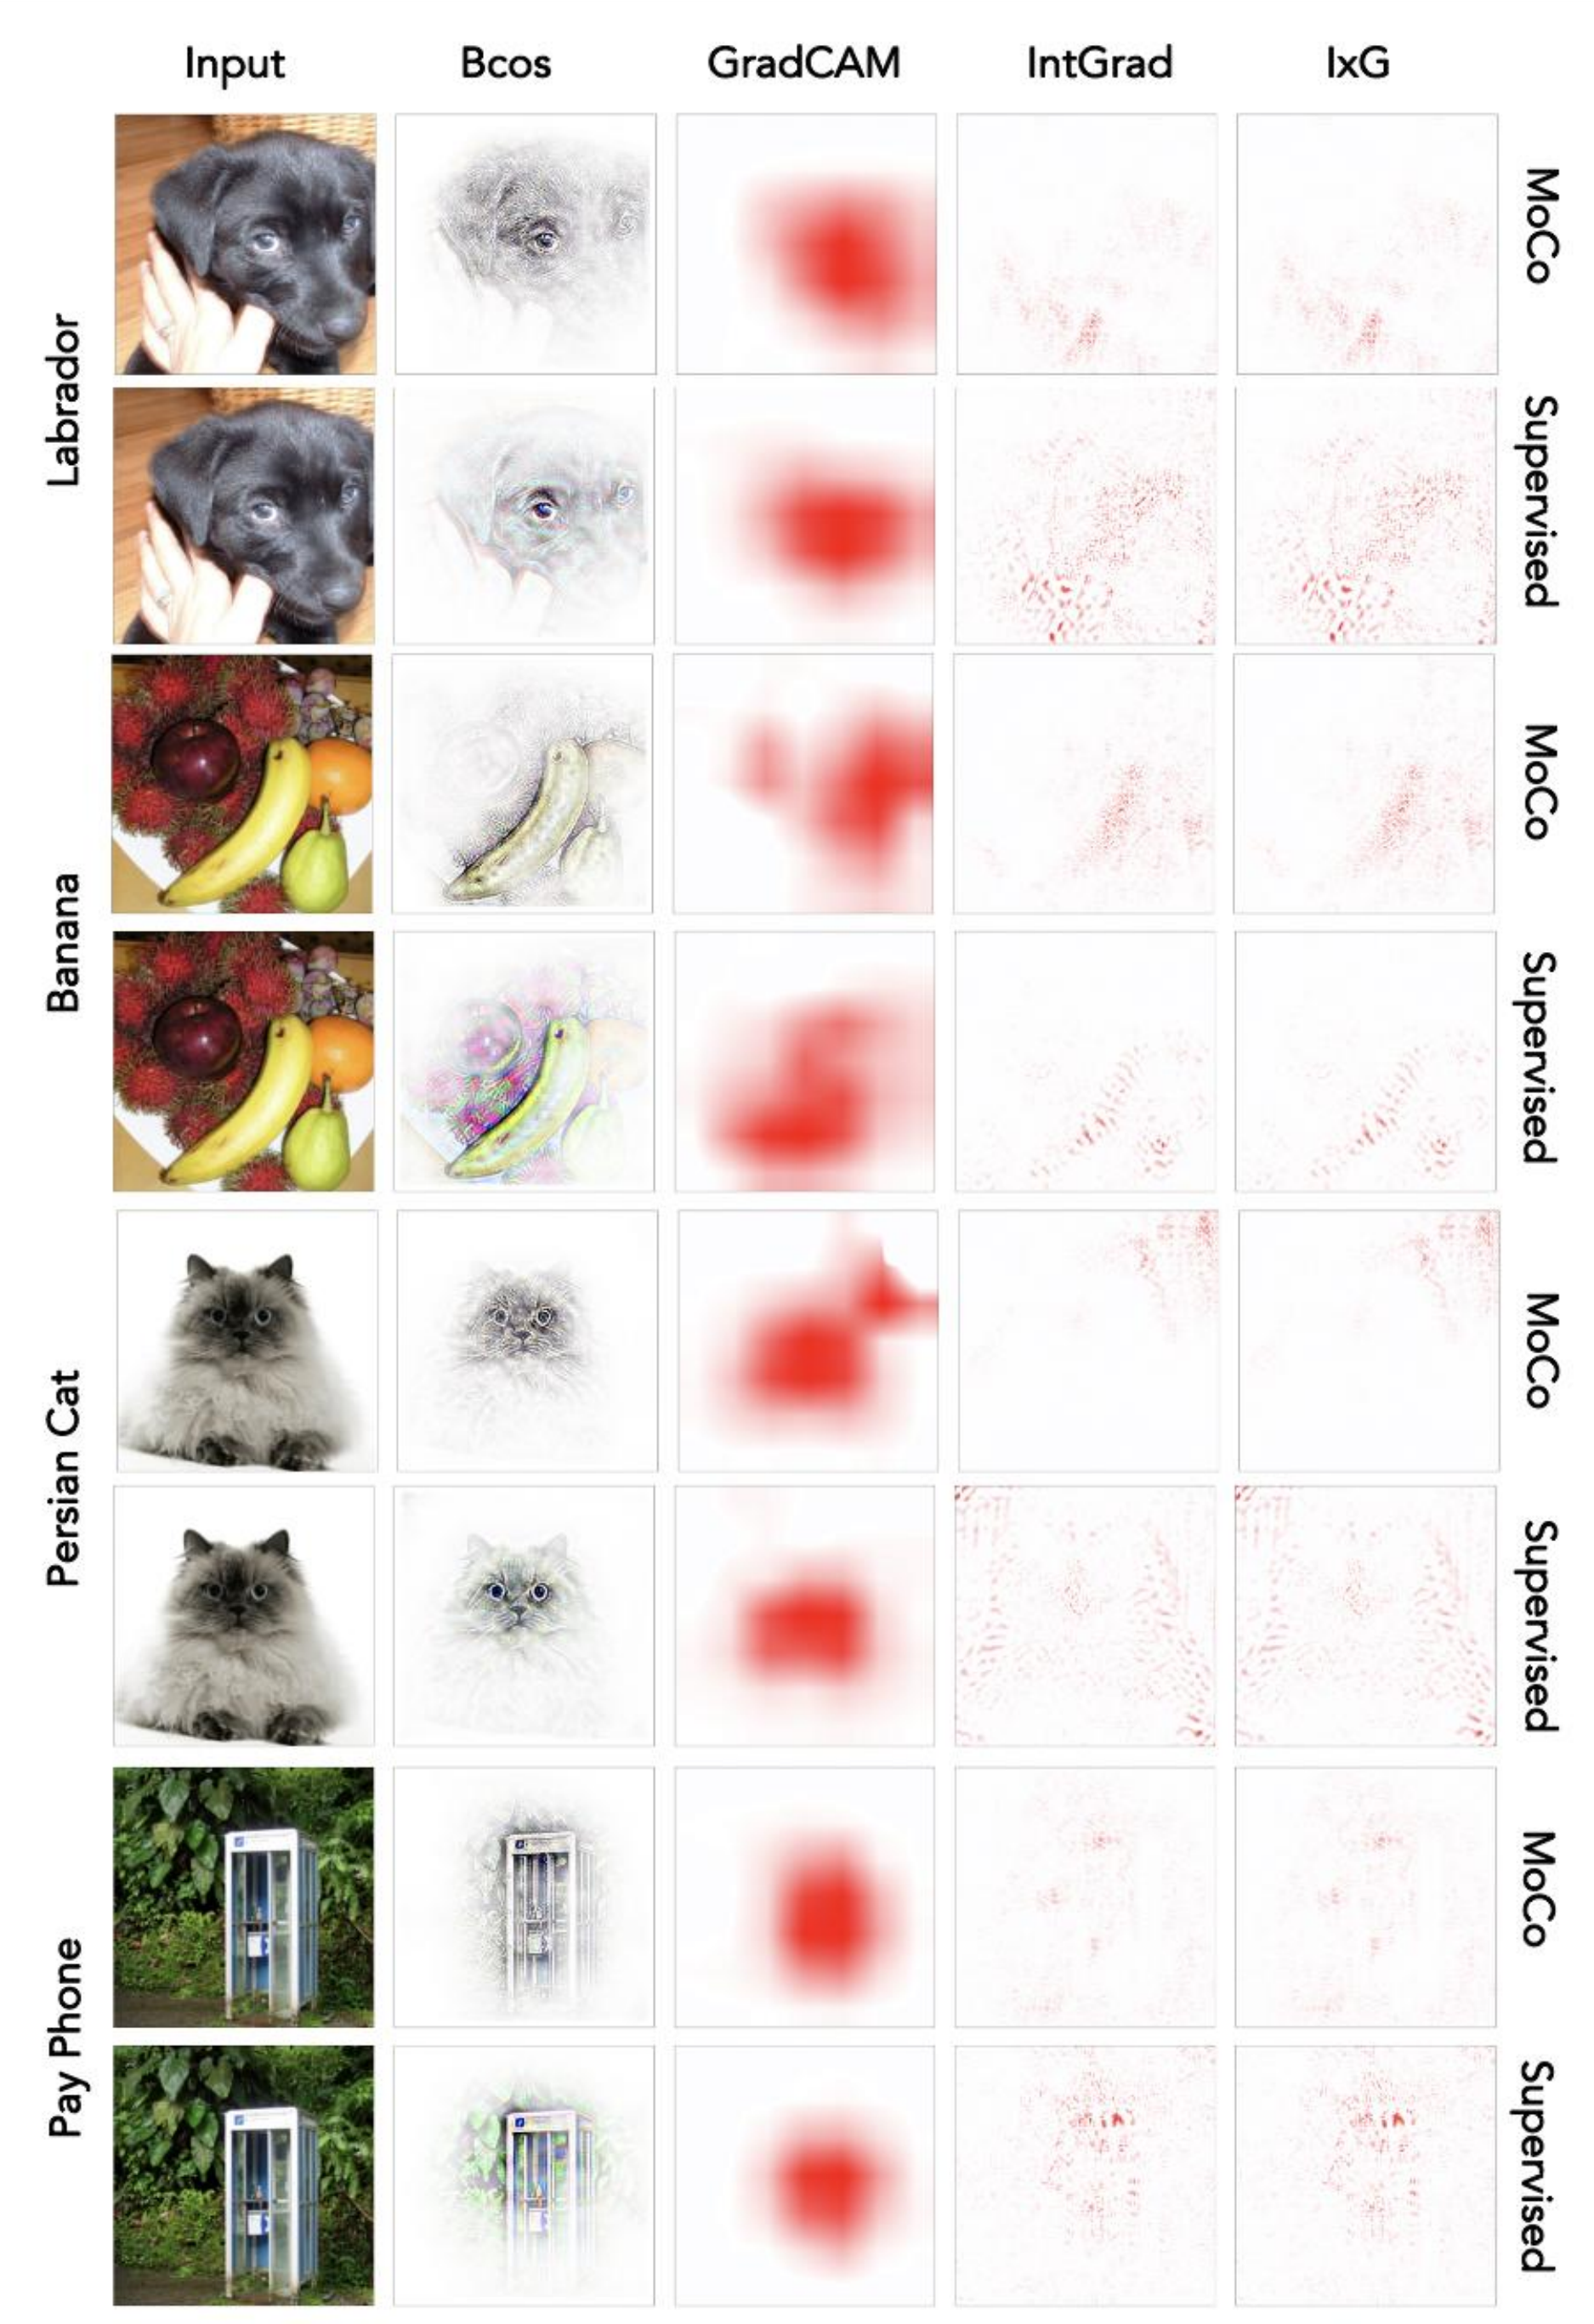}
\end{center}
    \vspace{-4mm}
    \caption
    { Qualitative results for different explanation methods for \textbf{\moco} and supervised \bcos models.
    \vspace{-1mm}
    }
   \label{fig:qual_bcos_moco}
\end{figure}

\begin{figure}
  \begin{center}
    \centering
        \includegraphics[width=0.85\linewidth]{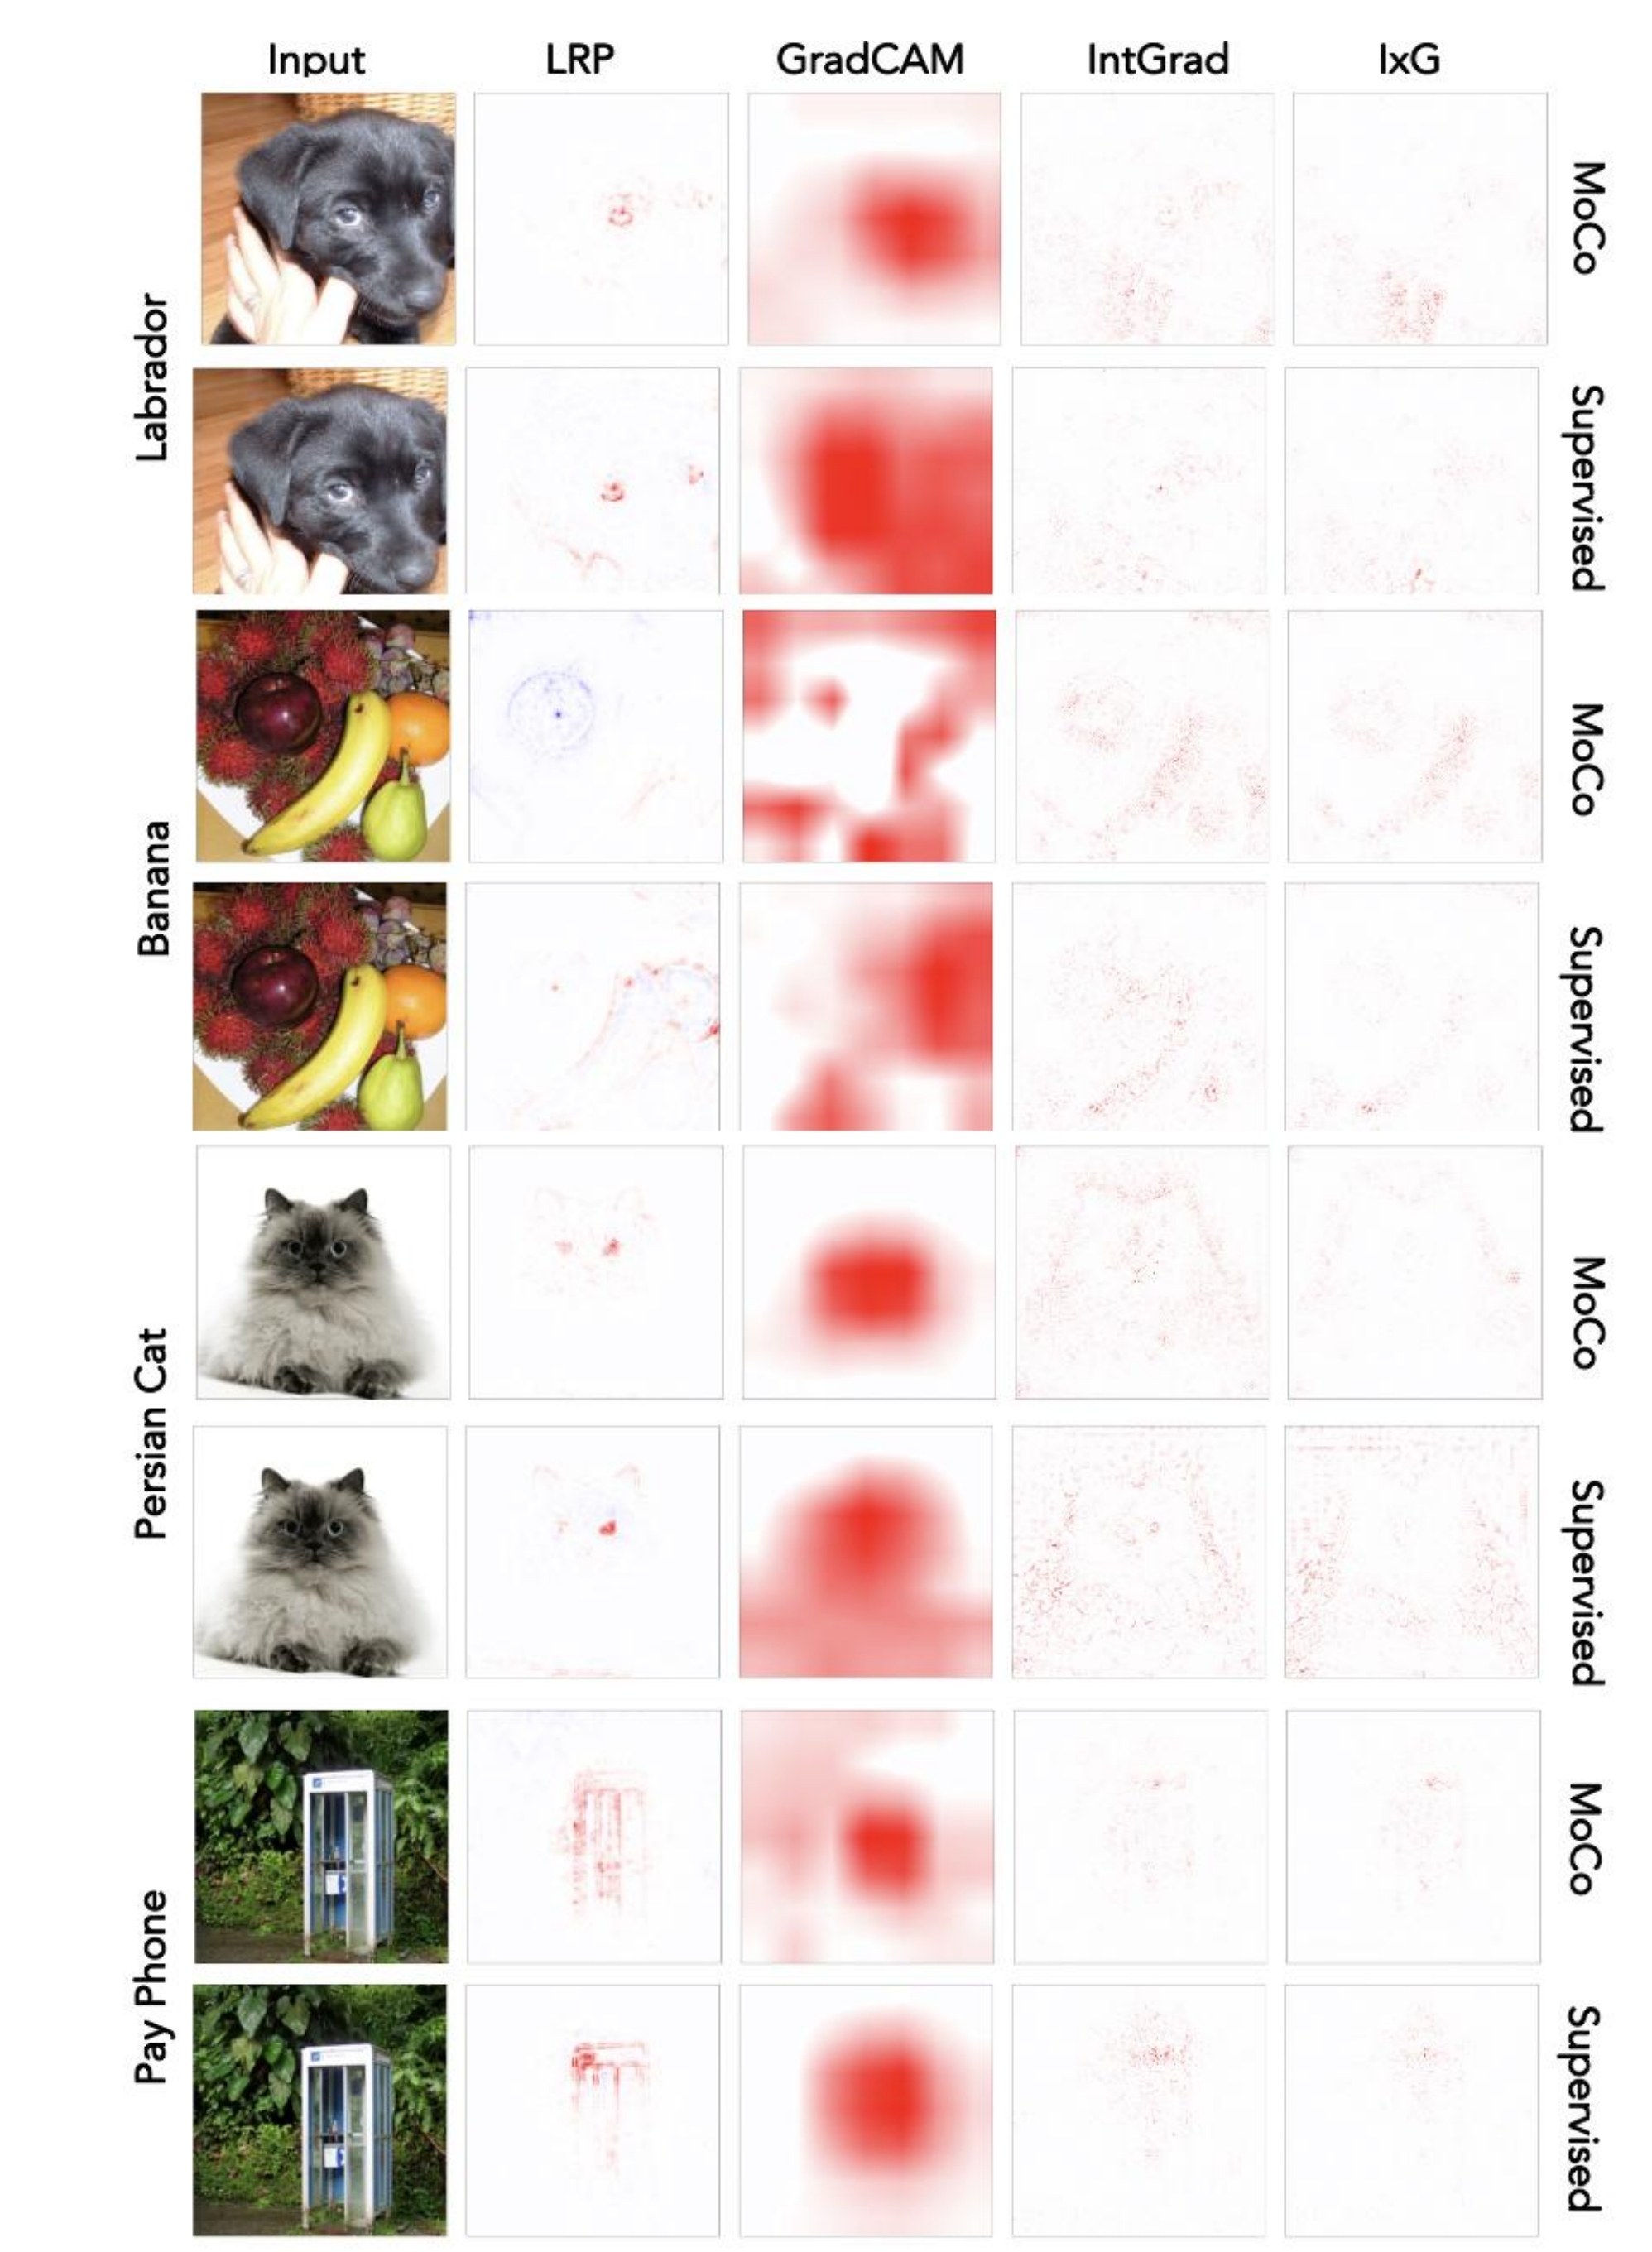}
\end{center}
    \vspace{-4mm}
    \caption
    {Qualitative results for different explanation methods for \textbf{\moco} and supervised conventional models.
    \vspace{-1mm}
    }
   \label{fig:qual_std_moco}
\end{figure}
